# Supplementary material for: Analyzing Adaptive Parameter Landscapes in Parameter Adaptation Methods for Differential Evolution
Source: arXiv:2009.12531 source file (2020-09-26)
Supplement: Supplementary file 1 [file supp.pdf]

# A Supplementary File for "Analyzing Adaptive Parameter Landscapes in Parameter Adaptation Methods for Differential Evolution"

Ryoji Tanabe
Yokohama National University
Yokohama, Japan
rt.ryoji.tanabe@gmail.com

## ABSTRACT

This paper is a supplementary file for "Analyzing Adaptive Parameter Landscapes in Parameter Adaptation Methods for Differential Evolution". **Note that missing figures are not typos. See Section 5.1 in the main paper for the reason why some figures are missing.**

**ACM Reference Format:**
Ryoji Tanabe. 2020. A Supplementary File for "Analyzing Adaptive Parameter Landscapes in Parameter Adaptation Methods for Differential Evolution". In *Proceedings of The Genetic and Evolutionary Computation Conference 2020 (GECCO '20).* ACM, New York, NY, USA, 47 pages. https://doi.org/10.1145/nnnnnnn.nnnnnnn

Permission to make digital or hard copies of part or all of this work for personal or classroom use is granted without fee provided that copies are not made or distributed for profit or commercial advantage and that copies bear this notice and the full citation on the first page. Copyrights for third-party components of this work must be honored. For all other uses, contact the owner/author(s).
*GECCO '20, July 8–12, 2020, Cancun, Mexico*
© 2020 Copyright held by the owner/author(s).
ACM ISBN 978-x-xxxx-xxxx-x/YY/MM.
https://doi.org/10.1145/nnnnnnn.nnnnnnn

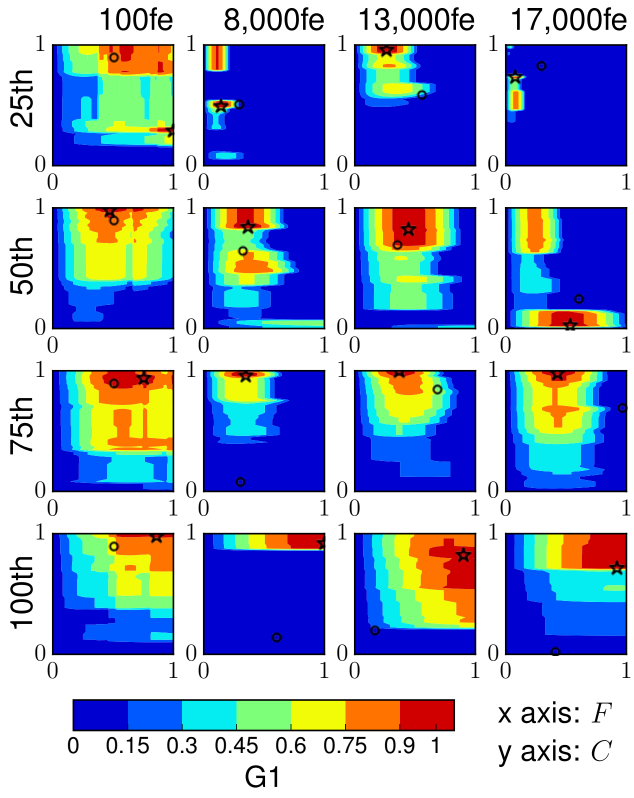


**Figure S.1: Contour maps of adaptive parameter landscapes in P-jDE on $f_1$ with $d = 20$.**

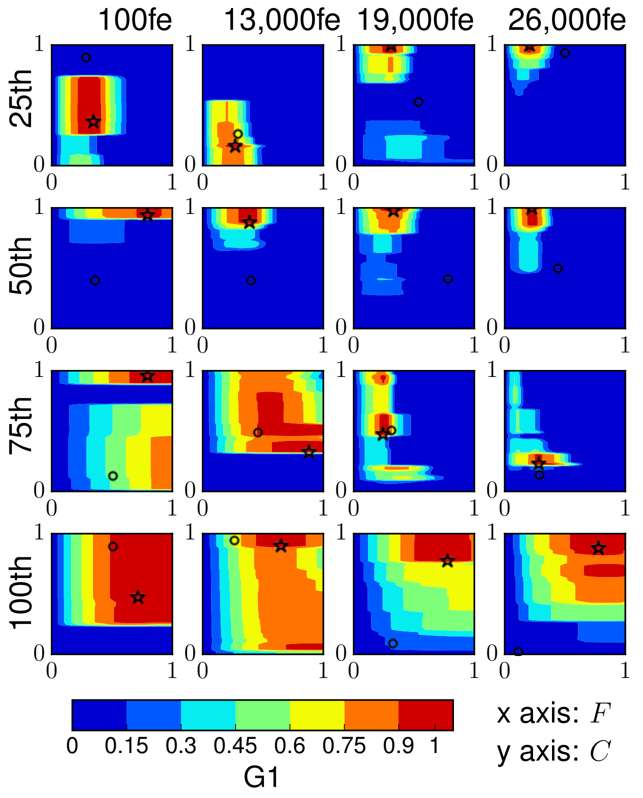


**Figure S.2: Contour maps of adaptive parameter landscapes in P-jDE on $f_2$ with $d = 20$.**

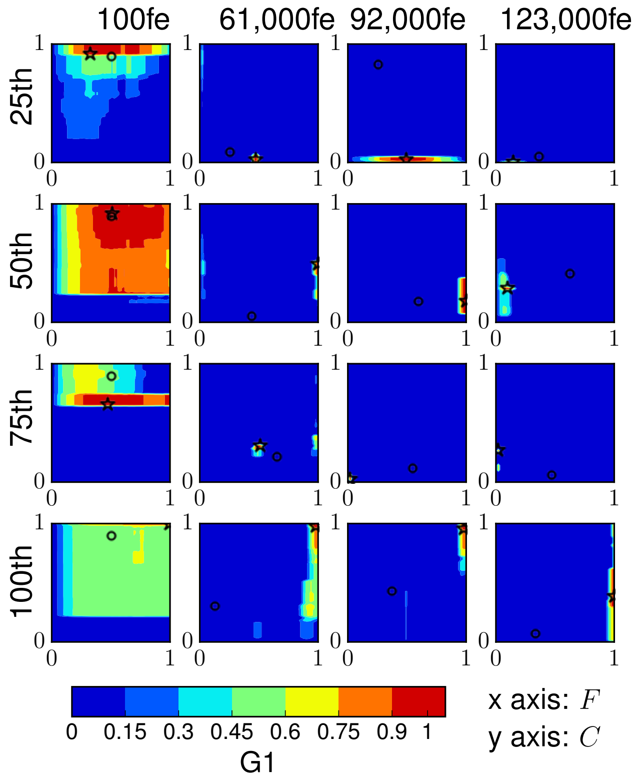


**Figure S.3: Contour maps of adaptive parameter landscapes in P-jDE on $f_3$ with $d = 20$.**

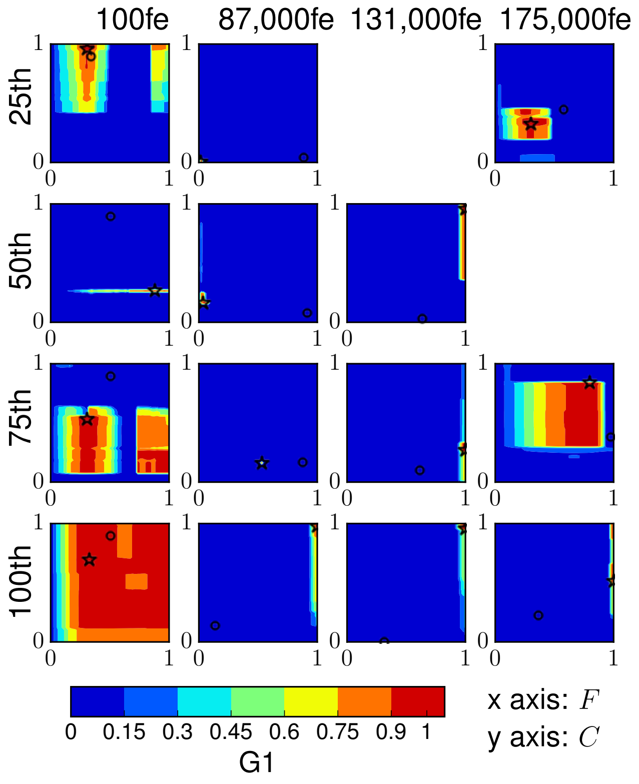


**Figure S.4: Contour maps of adaptive parameter landscapes in P-jDE on $f_4$ with $d = 20$.**

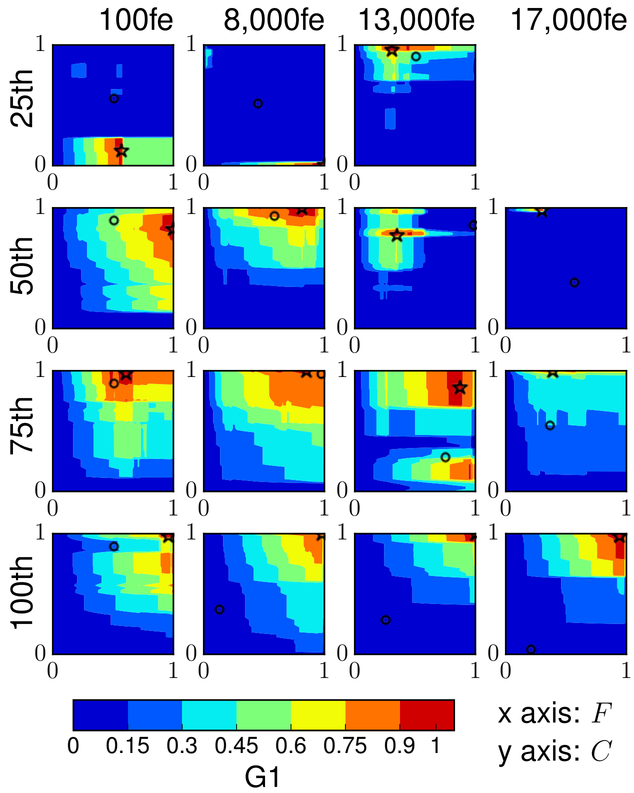


**Figure S.5: Contour maps of adaptive parameter landscapes in P-jDE on $f_5$ with $d = 20$.**

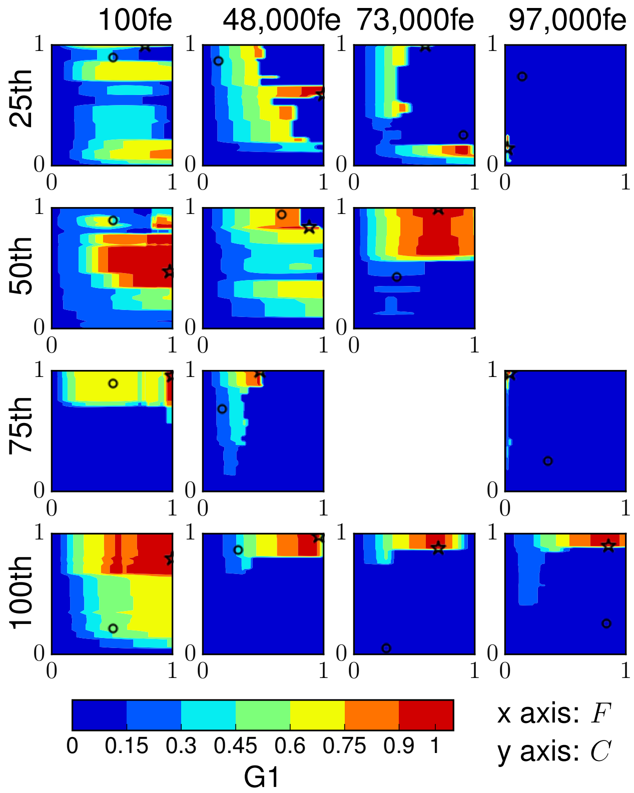


**Figure S.6: Contour maps of adaptive parameter landscapes in P-jDE on $f_6$ with $d = 20$.**

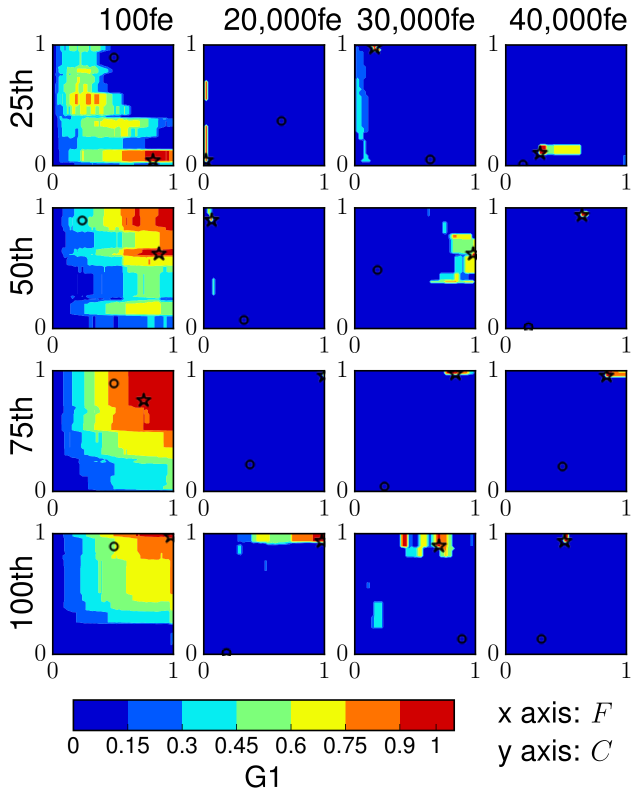


**Figure S.7: Contour maps of adaptive parameter landscapes in P-jDE on $f_7$ with $d = 20$.**

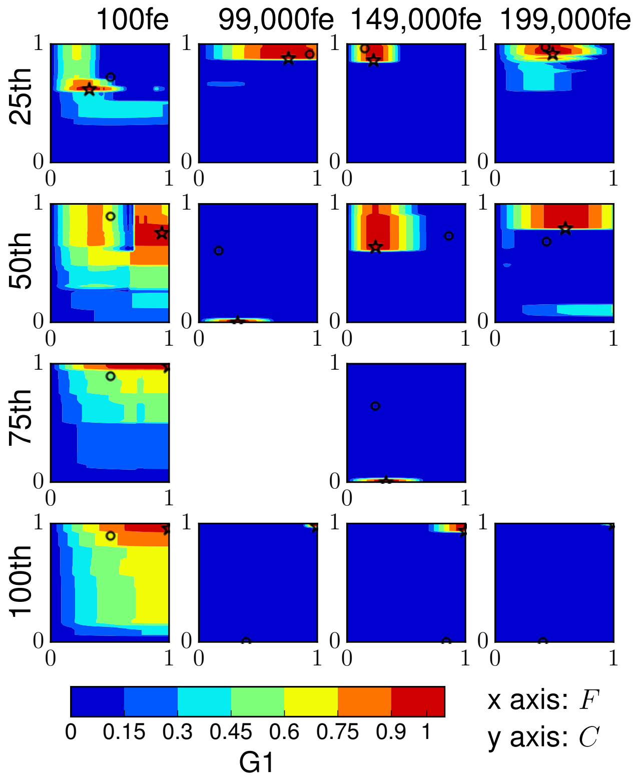


**Figure S.8: Contour maps of adaptive parameter landscapes in P-jDE on $f_8$ with $d = 20$.**

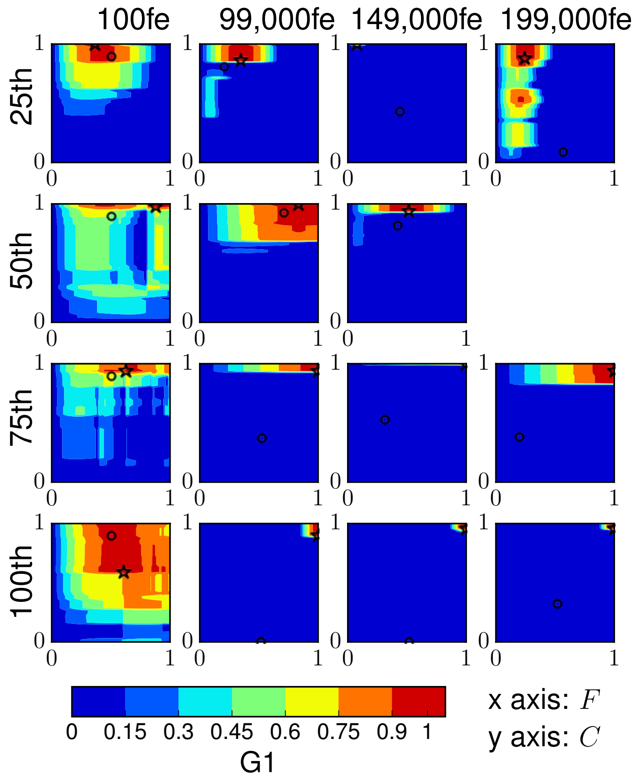


**Figure S.9: Contour maps of adaptive parameter landscapes in P-jDE on $f_9$ with $d = 20$.**

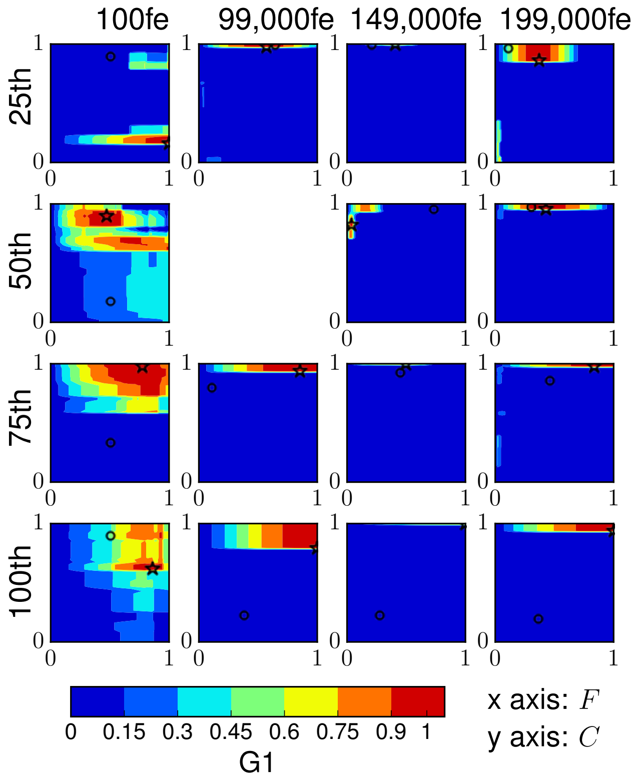


**Figure S.10: Contour maps of adaptive parameter landscapes in P-jDE on $f_{10}$ with $d = 20$.**

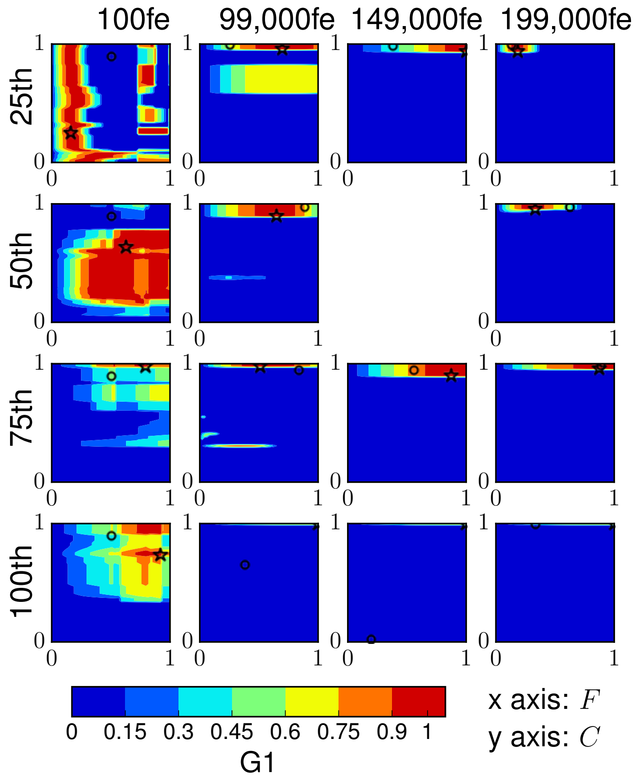


**Figure S.11: Contour maps of adaptive parameter landscapes in P-jDE on $f_{11}$ with $d = 20$.**

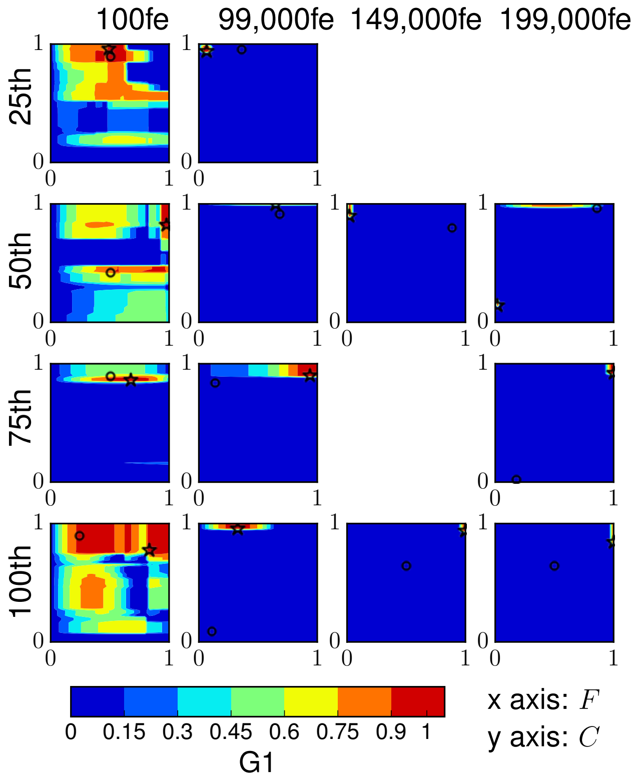


**Figure S.12: Contour maps of adaptive parameter landscapes in P-jDE on $f_{12}$ with $d = 20$.**

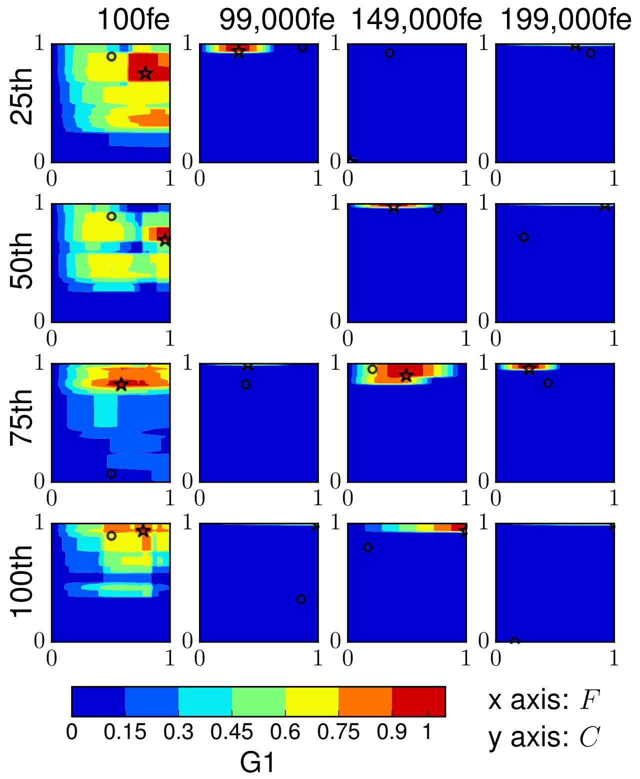


**Figure S.13: Contour maps of adaptive parameter landscapes in P-jDE on $f_{13}$ with $d = 20$.**

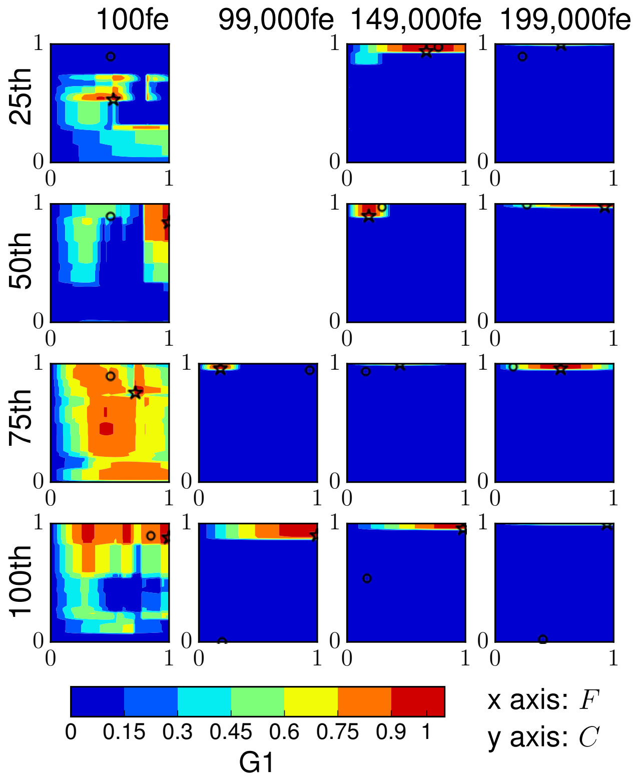


**Figure S.14: Contour maps of adaptive parameter landscapes in P-jDE on $f_{14}$ with $d = 20$.**

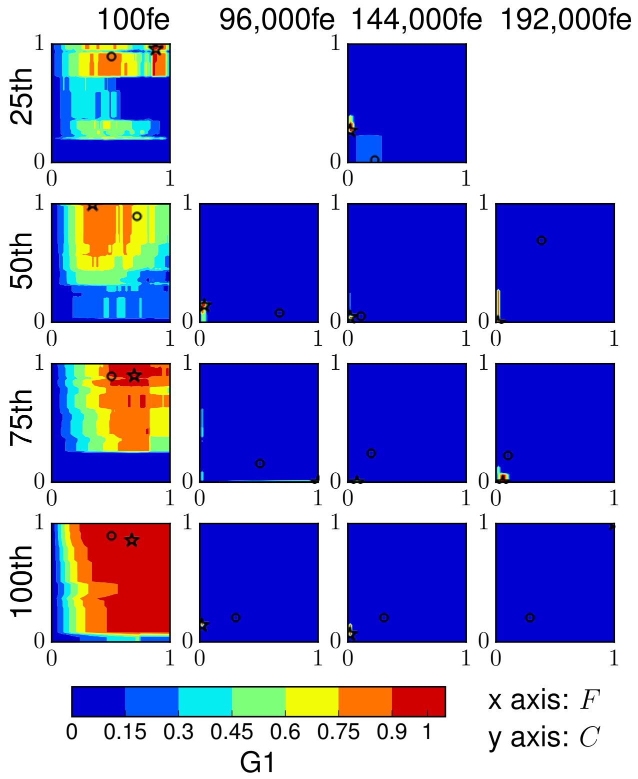


**Figure S.15: Contour maps of adaptive parameter landscapes in P-jDE on $f_{15}$ with $d = 20$.**

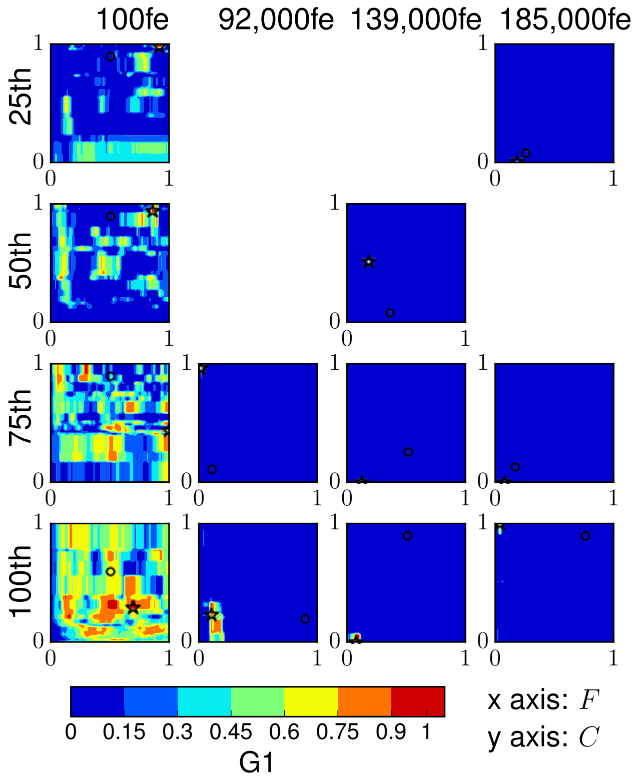


**Figure S.16: Contour maps of adaptive parameter landscapes in P-jDE on $f_{16}$ with $d = 20$.**

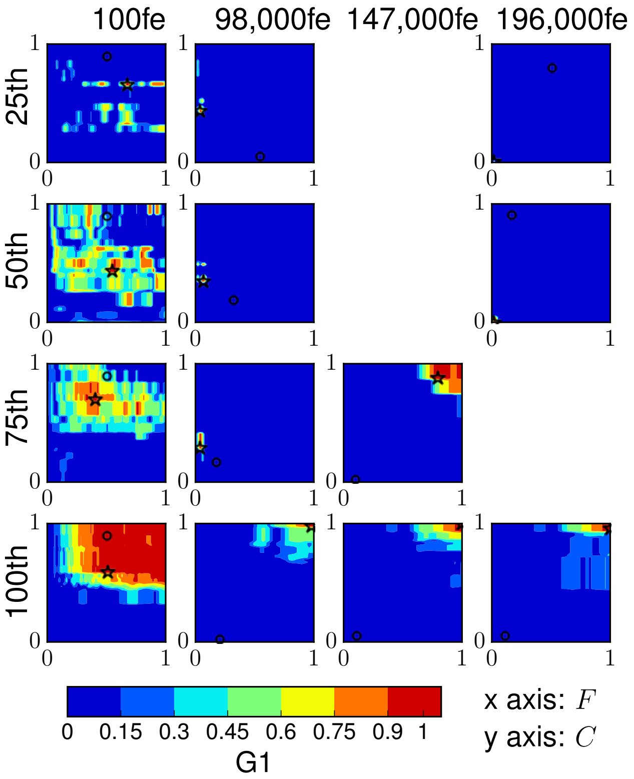


**Figure S.17: Contour maps of adaptive parameter landscapes in P-jDE on $f_{17}$ with $d = 20$.**

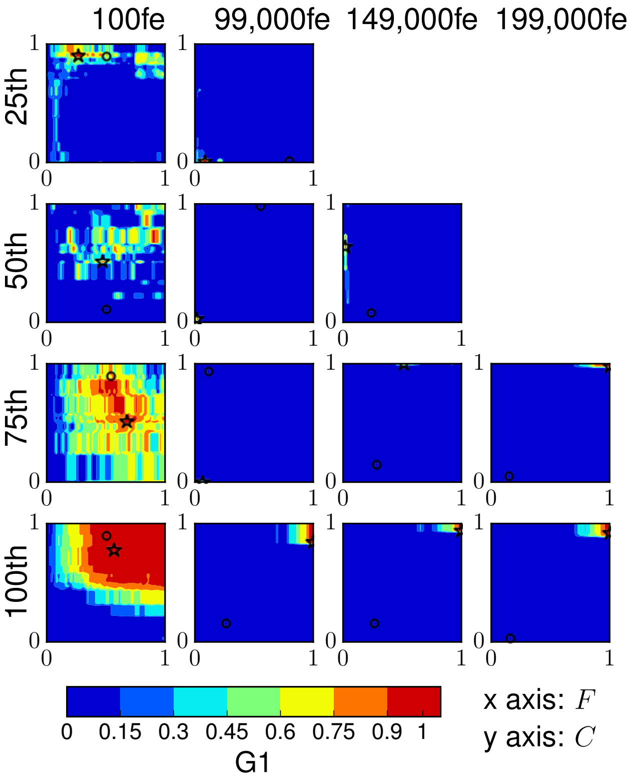


**Figure S.18: Contour maps of adaptive parameter landscapes in P-jDE on $f_{18}$ with $d = 20$.**

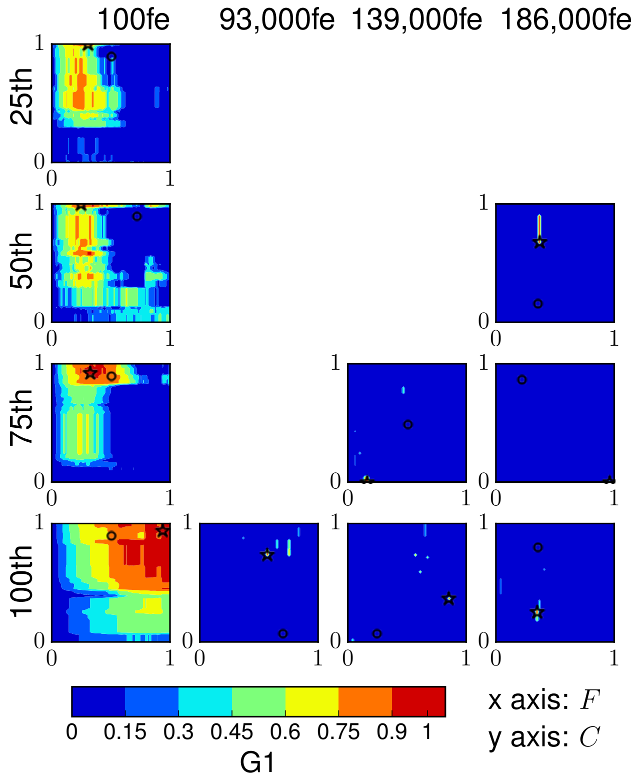


**Figure S.19: Contour maps of adaptive parameter landscapes in P-jDE on $f_{19}$ with $d = 20$.**

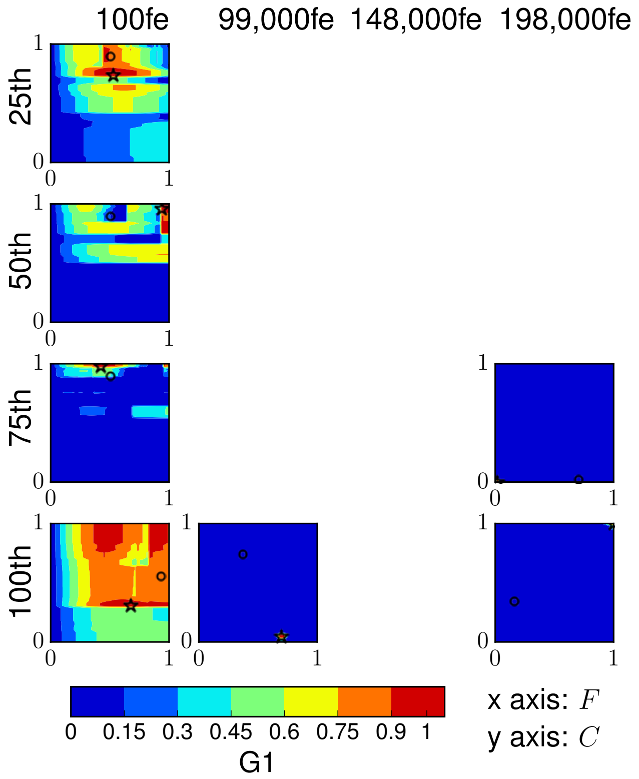


**Figure S.20: Contour maps of adaptive parameter landscapes in P-jDE on $f_{20}$ with $d = 20$.**

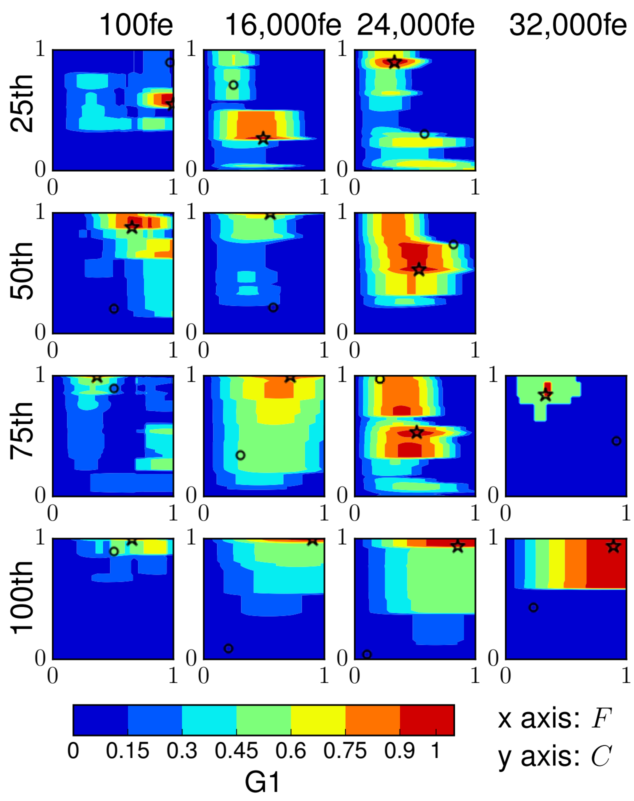


**Figure S.21: Contour maps of adaptive parameter landscapes in P-jDE on $f_{21}$ with $d = 20$.**

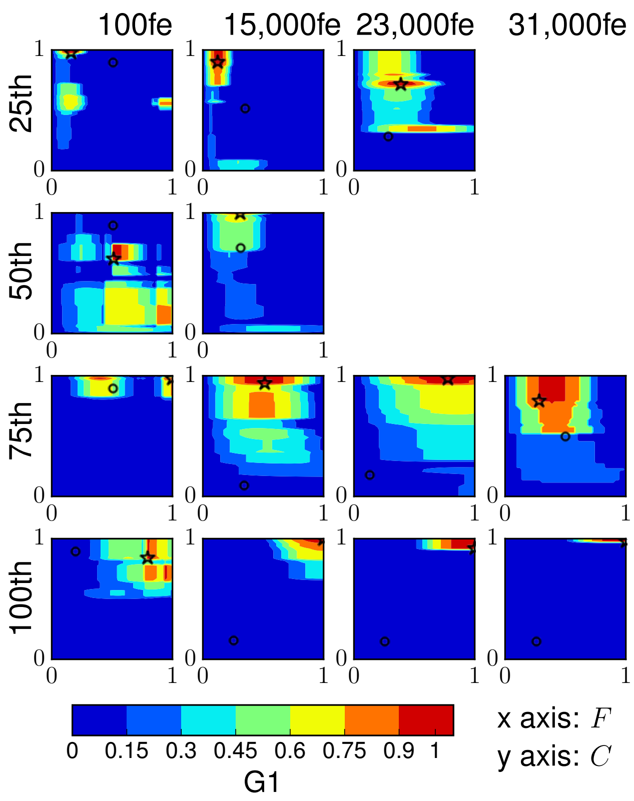


**Figure S.22: Contour maps of adaptive parameter landscapes in P-jDE on $f_{22}$ with $d = 20$.**

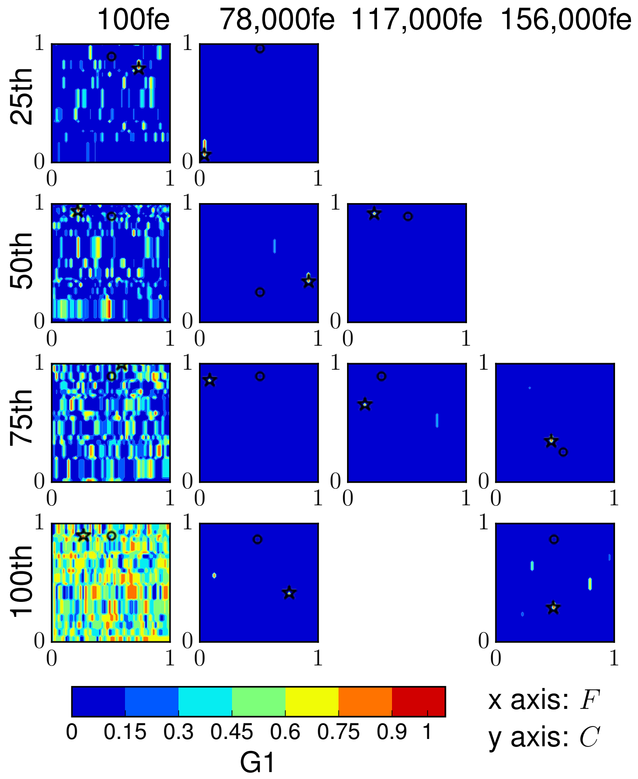


**Figure S.23: Contour maps of adaptive parameter landscapes in P-jDE on $f_{23}$ with $d = 20$.**

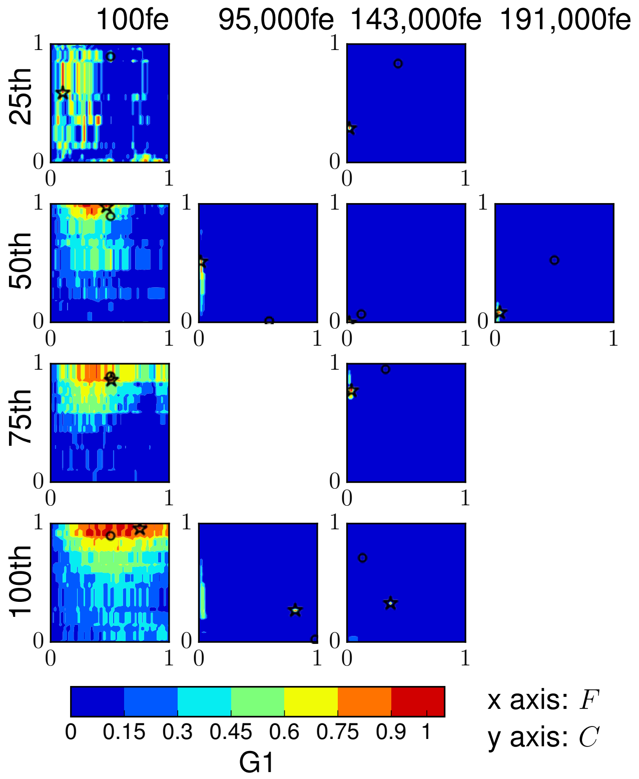


**Figure S.24: Contour maps of adaptive parameter landscapes in P-jDE on $f_{24}$ with $d = 20$.**

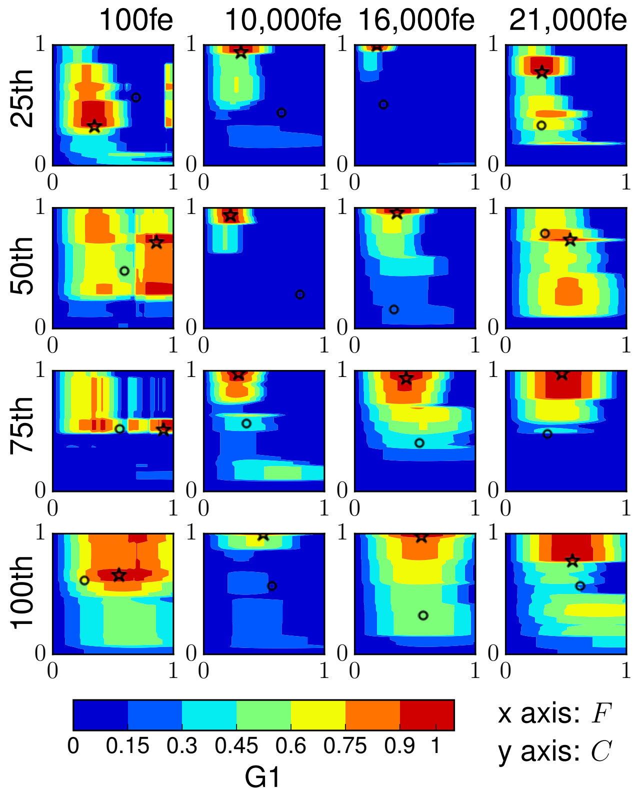


**Figure S.25: Contour maps of adaptive parameter landscapes in P-JADE on $f_1$ with $d = 20$.**

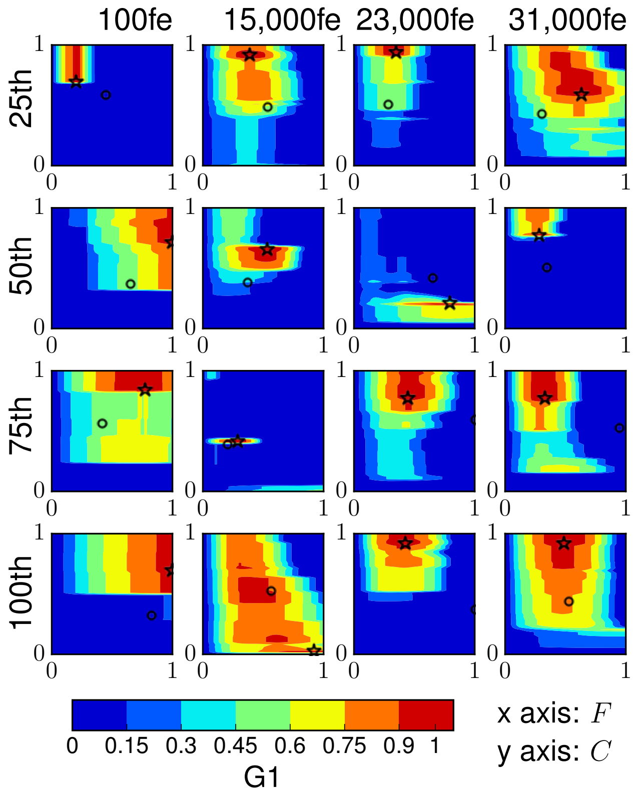


**Figure S.26: Contour maps of adaptive parameter landscapes in P-JADE on $f_2$ with $d = 20$.**

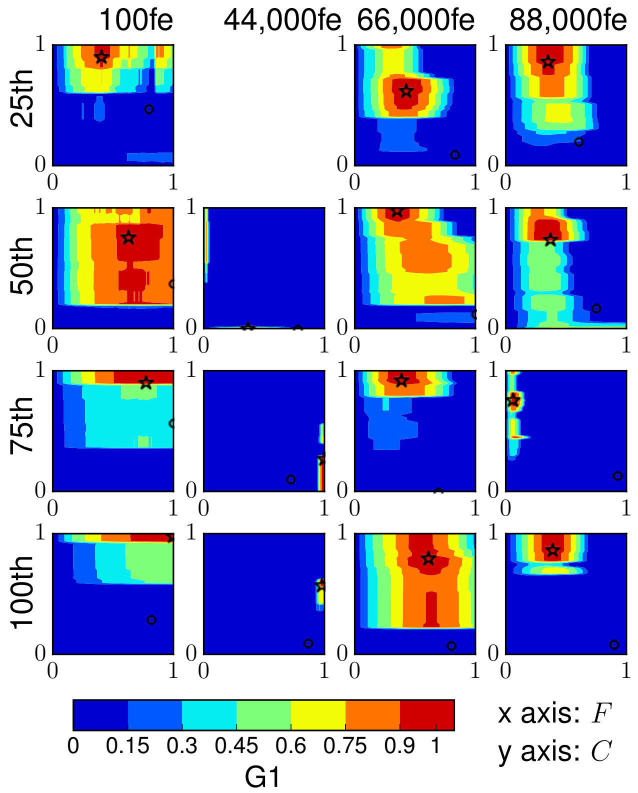


**Figure S.27: Contour maps of adaptive parameter landscapes in P-JADE on $f_3$ with $d = 20$.**

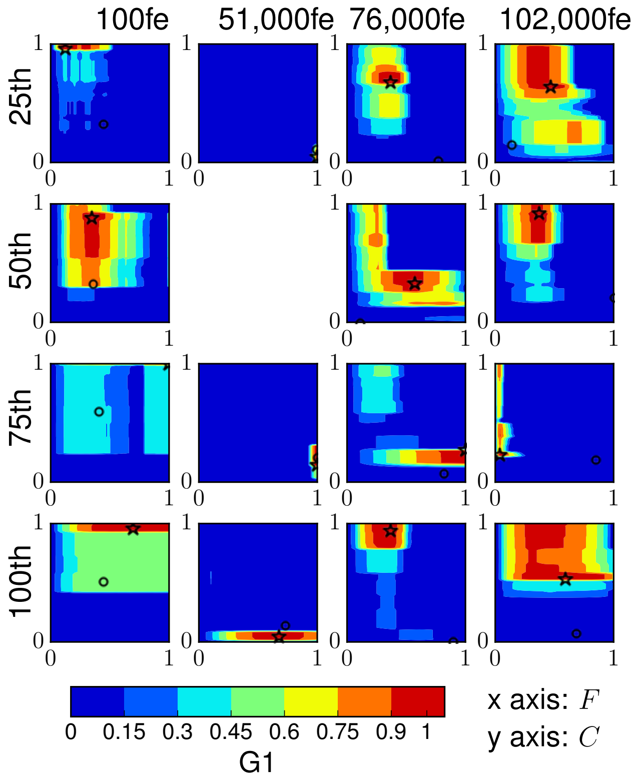


**Figure S.28: Contour maps of adaptive parameter landscapes in P-JADE on $f_4$ with $d = 20$.**

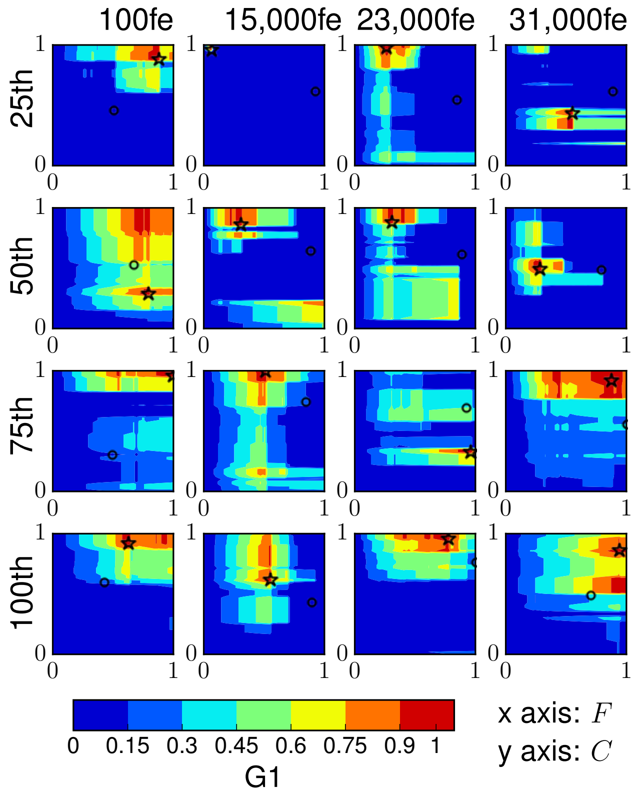


**Figure S.29: Contour maps of adaptive parameter landscapes in P-JADE on $f_5$ with $d = 20$.**

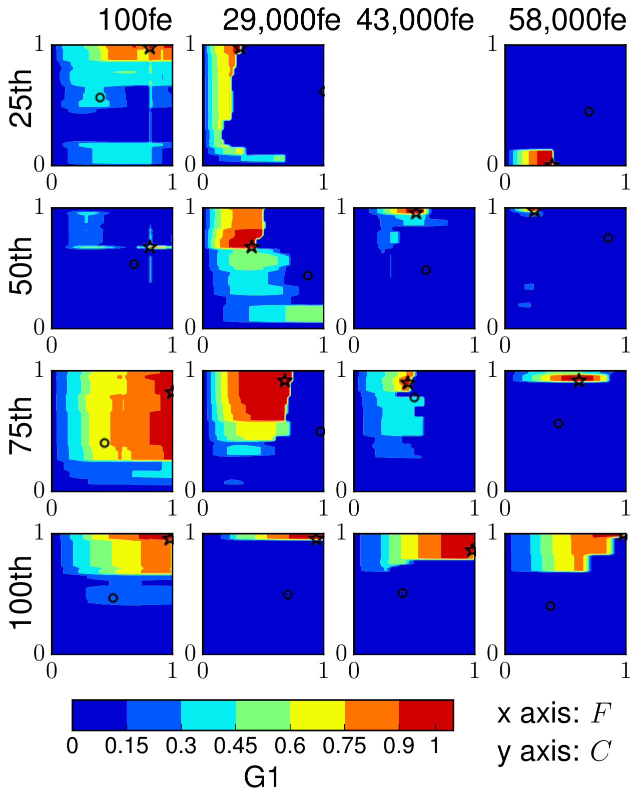


**Figure S.30: Contour maps of adaptive parameter landscapes in P-JADE on $f_6$ with $d = 20$.**

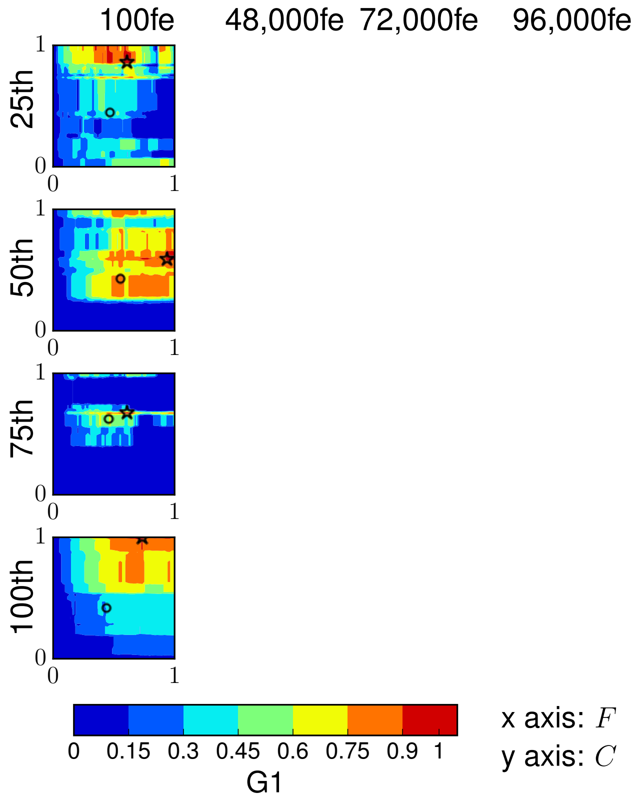


**Figure S.31: Contour maps of adaptive parameter landscapes in P-JADE on $f_7$ with $d = 20$.**

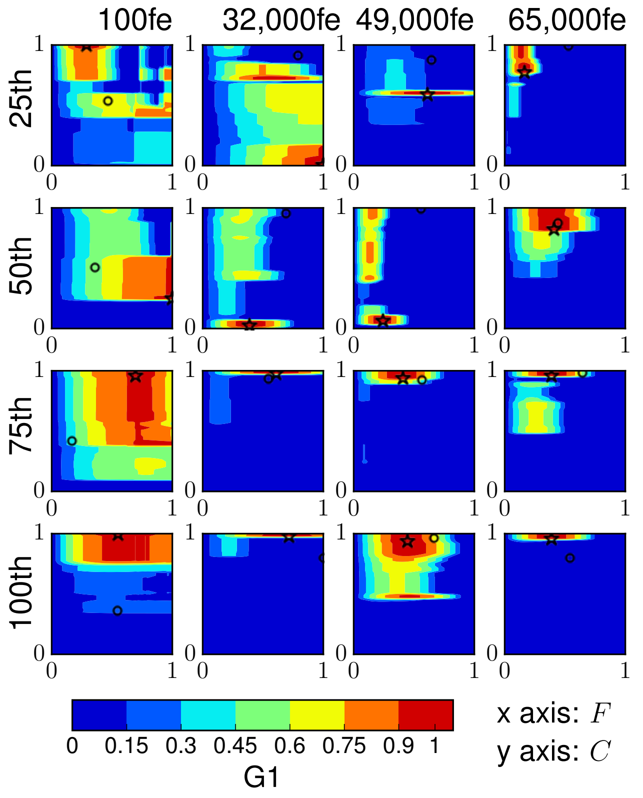


**Figure S.32: Contour maps of adaptive parameter landscapes in P-JADE on $f_8$ with $d = 20$.**

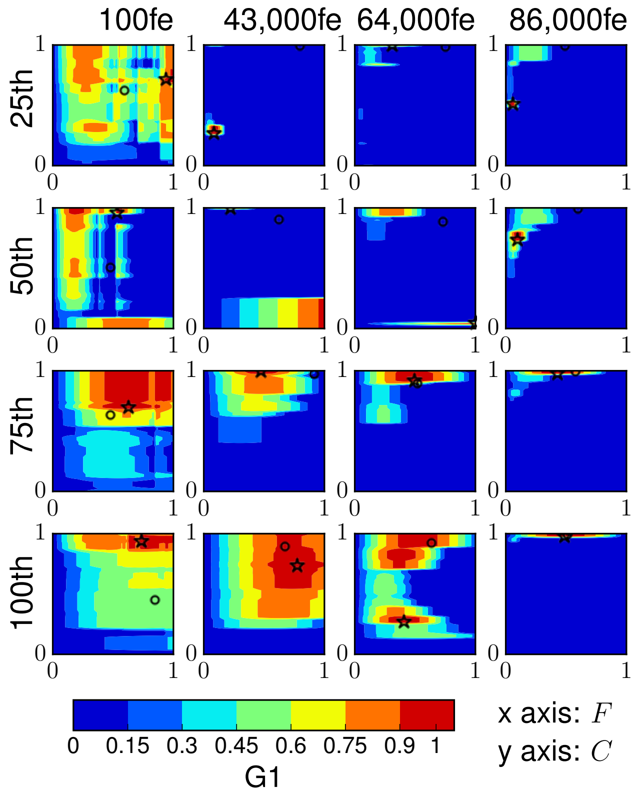


**Figure S.33: Contour maps of adaptive parameter landscapes in P-JADE on $f_9$ with $d = 20$.**

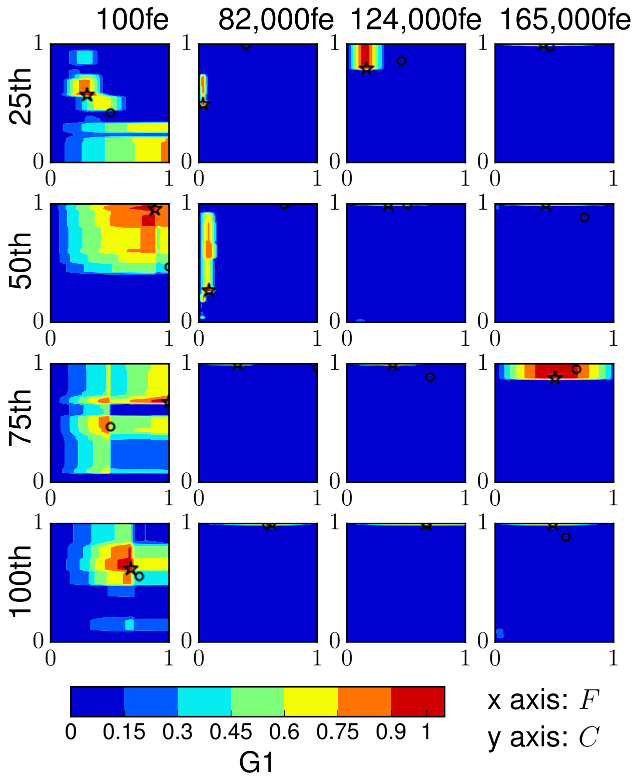


**Figure S.34: Contour maps of adaptive parameter landscapes in P-JADE on $f_{10}$ with $d = 20$.**

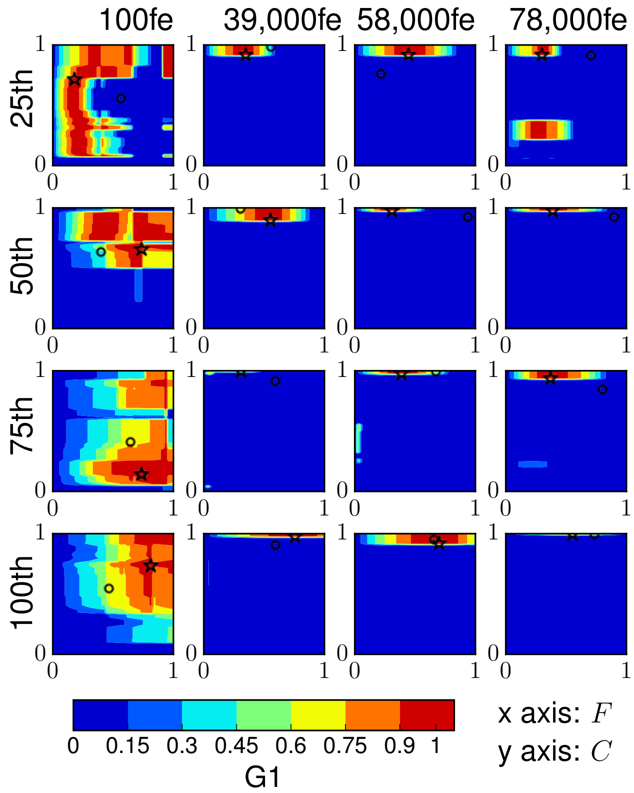


**Figure S.35: Contour maps of adaptive parameter landscapes in P-JADE on $f_{11}$ with $d = 20$.**

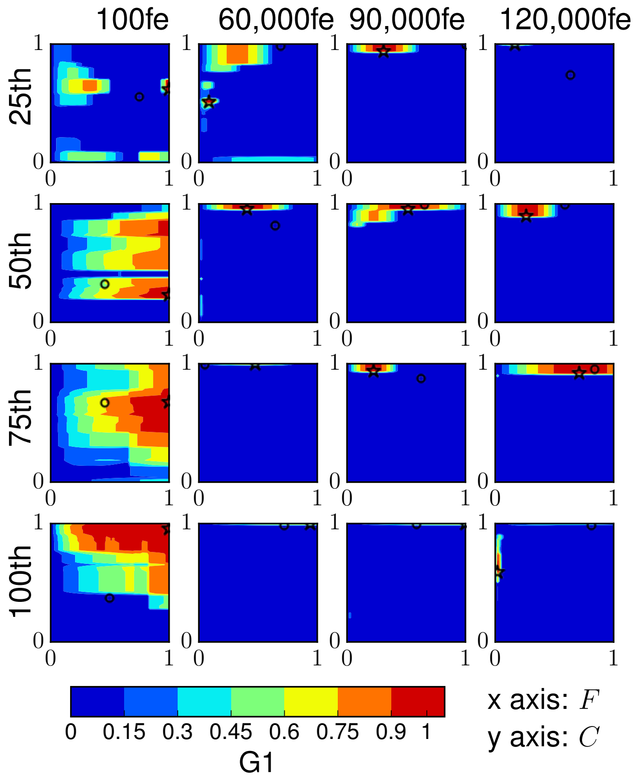


**Figure S.36: Contour maps of adaptive parameter landscapes in P-JADE on $f_{12}$ with $d = 20$.**

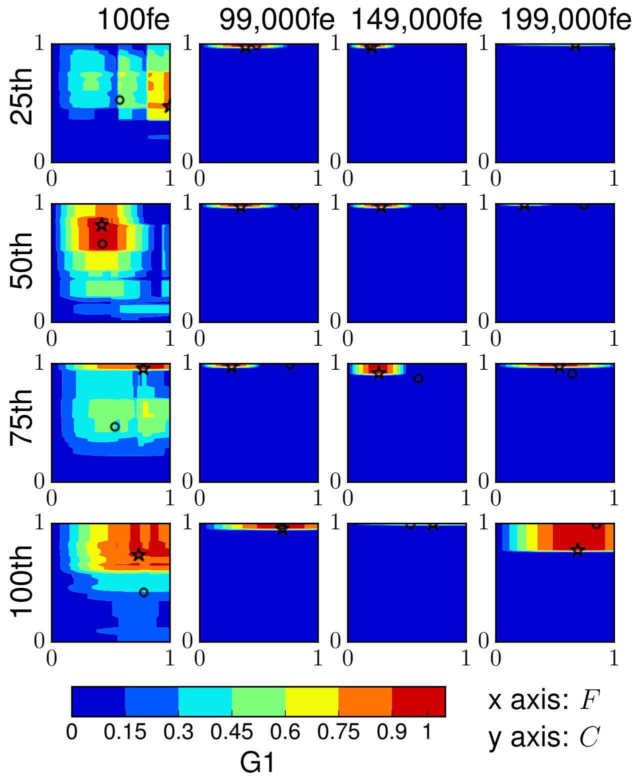


**Figure S.37: Contour maps of adaptive parameter landscapes in P-JADE on $f_{13}$ with $d = 20$.**

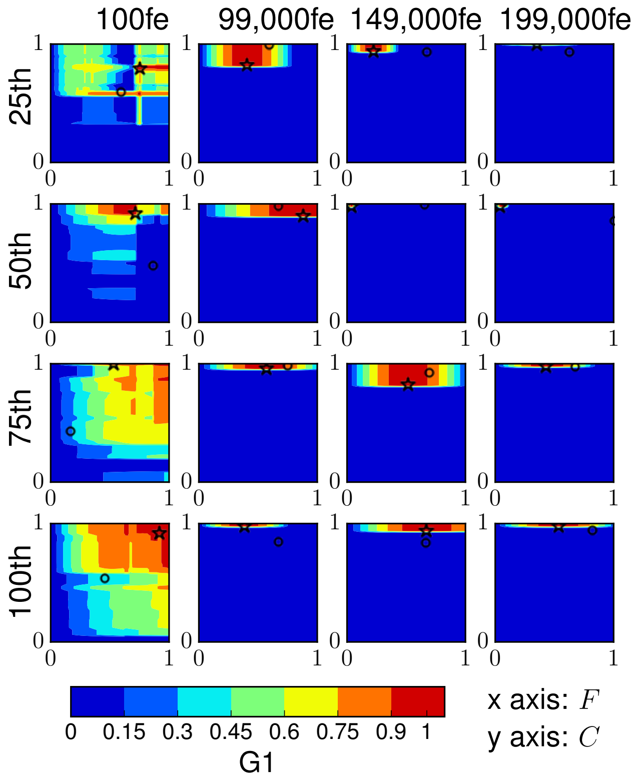


**Figure S.38: Contour maps of adaptive parameter landscapes in P-JADE on $f_{14}$ with $d = 20$.**

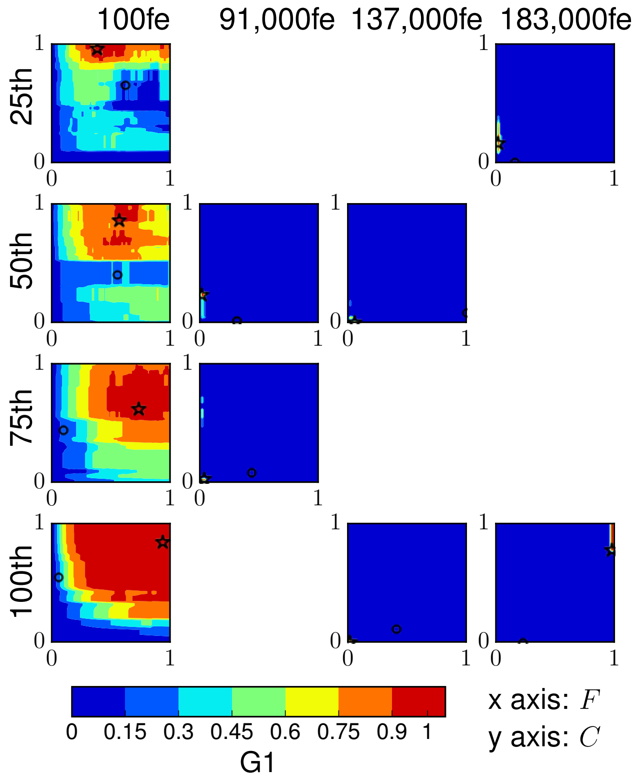


**Figure S.39: Contour maps of adaptive parameter landscapes in P-JADE on $f_{15}$ with $d = 20$.**

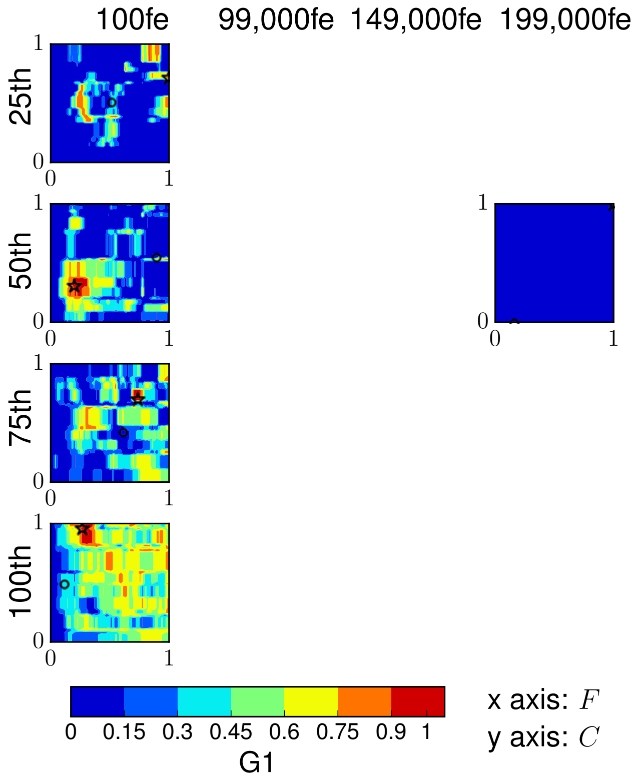


**Figure S.40: Contour maps of adaptive parameter landscapes in P-JADE on $f_{16}$ with $d = 20$.**

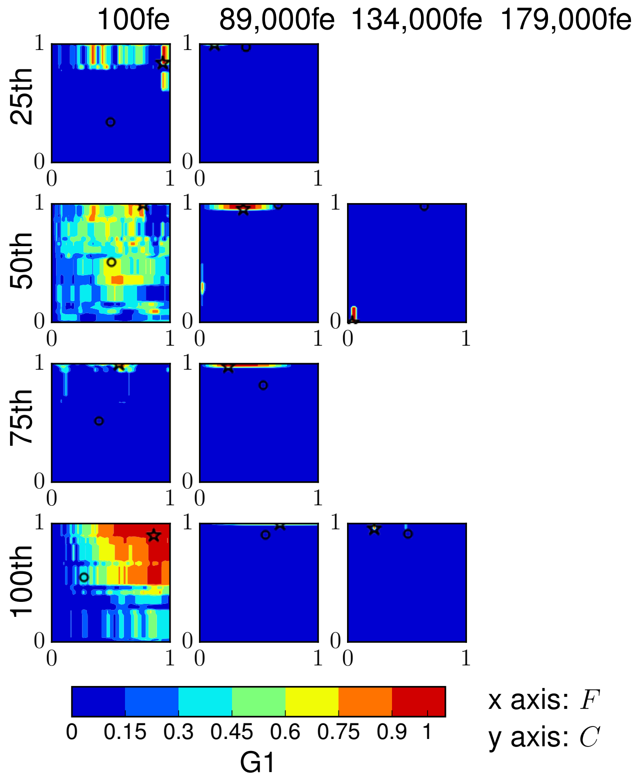


**Figure S.41: Contour maps of adaptive parameter landscapes in P-JADE on $f_{17}$ with $d = 20$.**

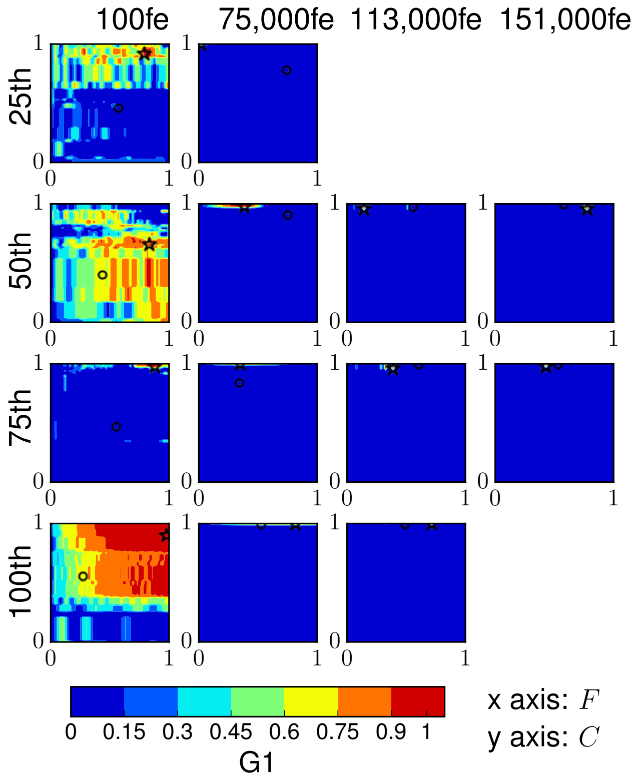


**Figure S.42: Contour maps of adaptive parameter landscapes in P-JADE on $f_{18}$ with $d = 20$.**

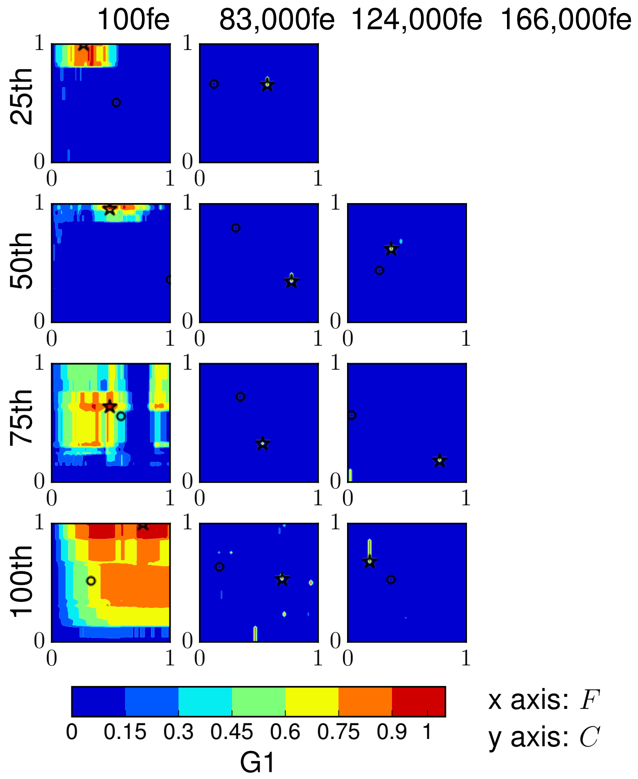


**Figure S.43: Contour maps of adaptive parameter landscapes in P-JADE on $f_{19}$ with $d = 20$.**

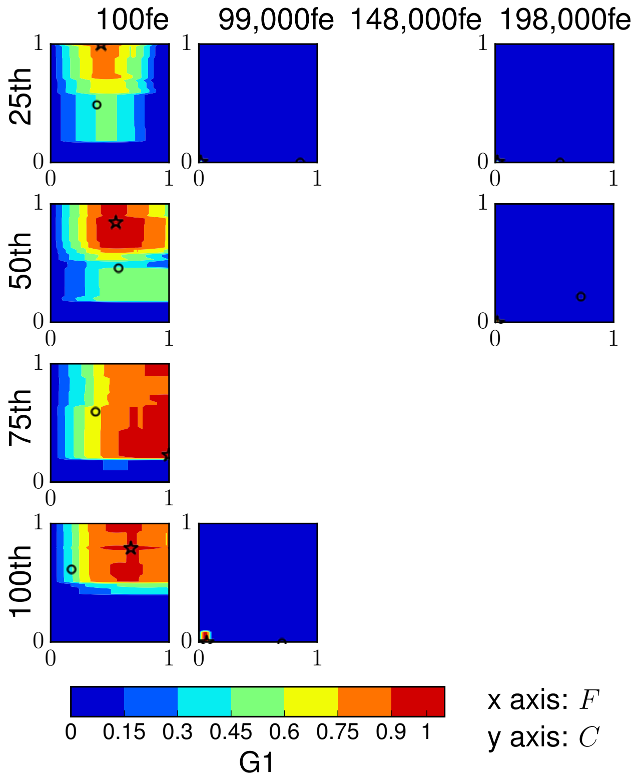


**Figure S.44: Contour maps of adaptive parameter landscapes in P-JADE on $f_{20}$ with $d = 20$.**

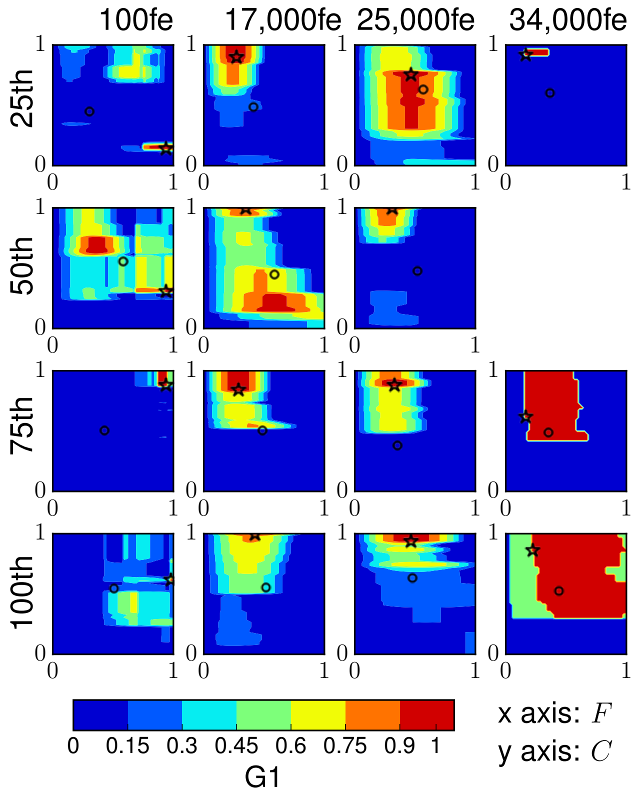


**Figure S.45: Contour maps of adaptive parameter landscapes in P-JADE on $f_{21}$ with $d = 20$.**

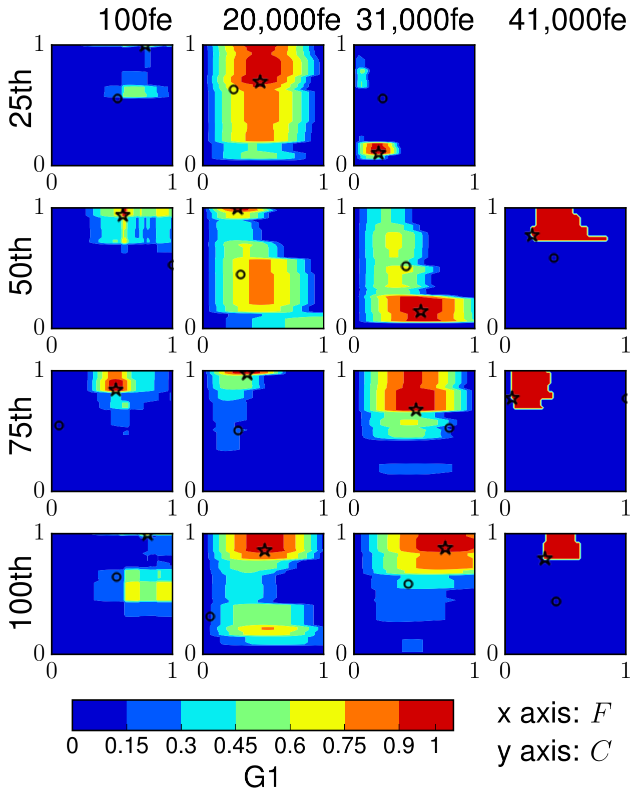


**Figure S.46: Contour maps of adaptive parameter landscapes in P-JADE on $f_{22}$ with $d = 20$.**

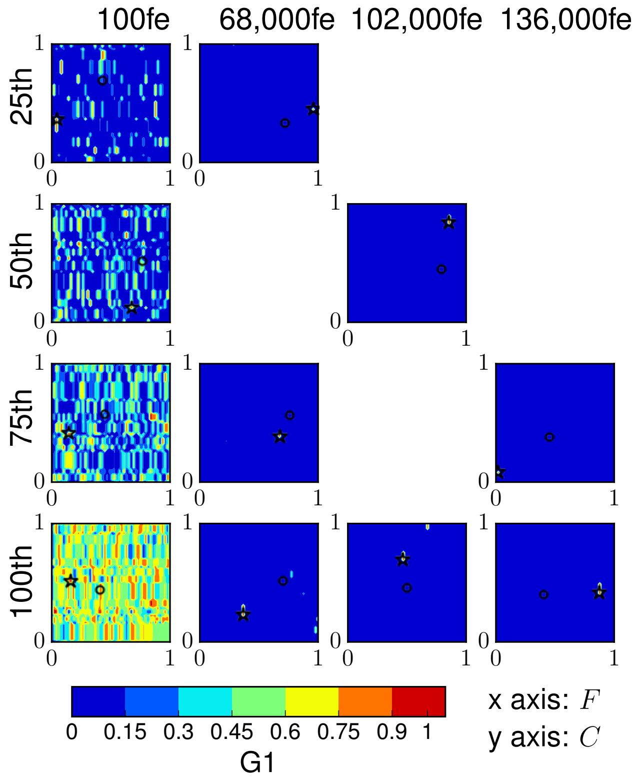


**Figure S.47: Contour maps of adaptive parameter landscapes in P-JADE on $f_{23}$ with $d = 20$.**

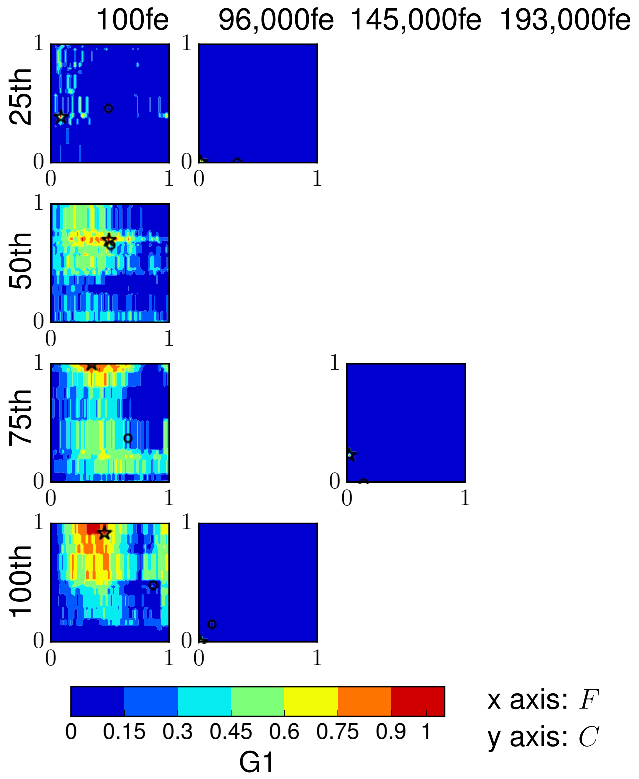


**Figure S.48: Contour maps of adaptive parameter landscapes in P-JADE on $f_{24}$ with $d = 20$.**

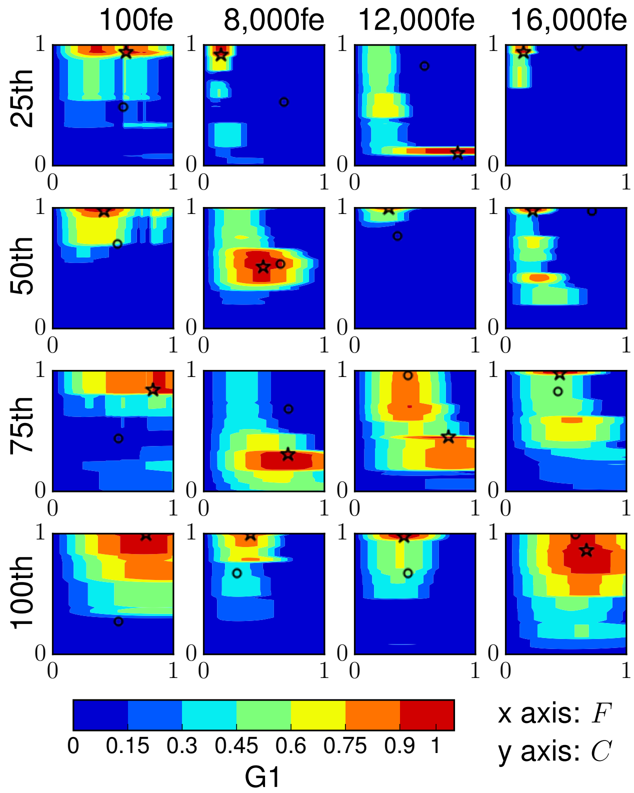


**Figure S.49: Contour maps of adaptive parameter landscapes in P-SHADE on $f_1$ with $d = 20$.**

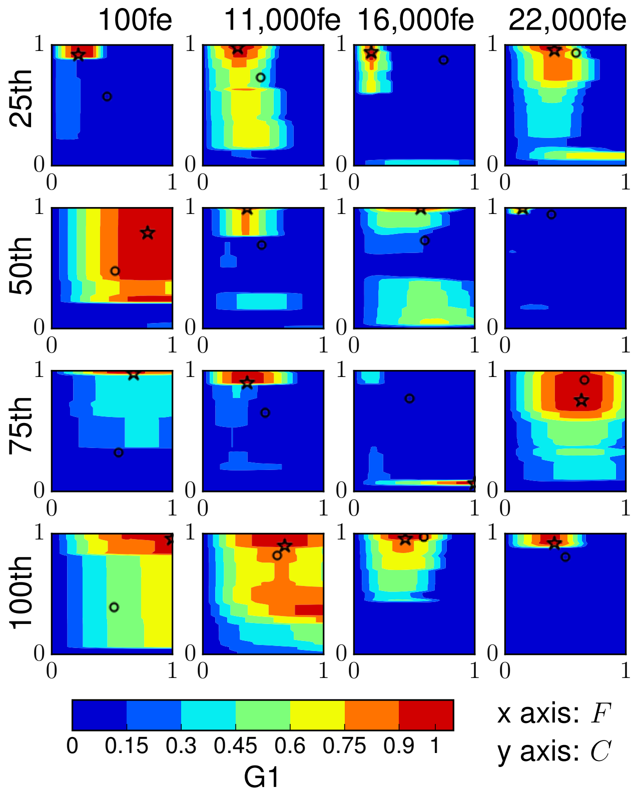


**Figure S.50: Contour maps of adaptive parameter landscapes in P-SHADE on $f_2$ with $d = 20$.**

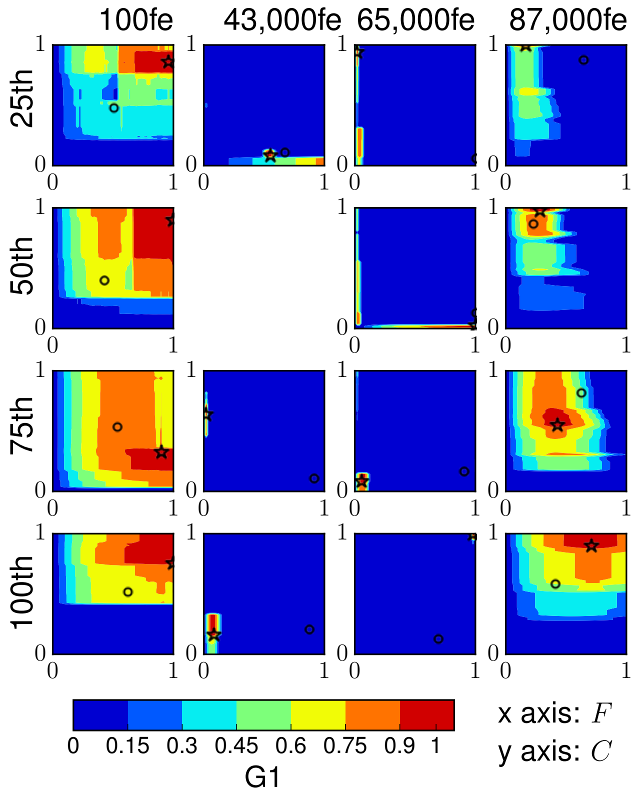


**Figure S.51: Contour maps of adaptive parameter landscapes in P-SHADE on $f_3$ with $d$ = 20.**

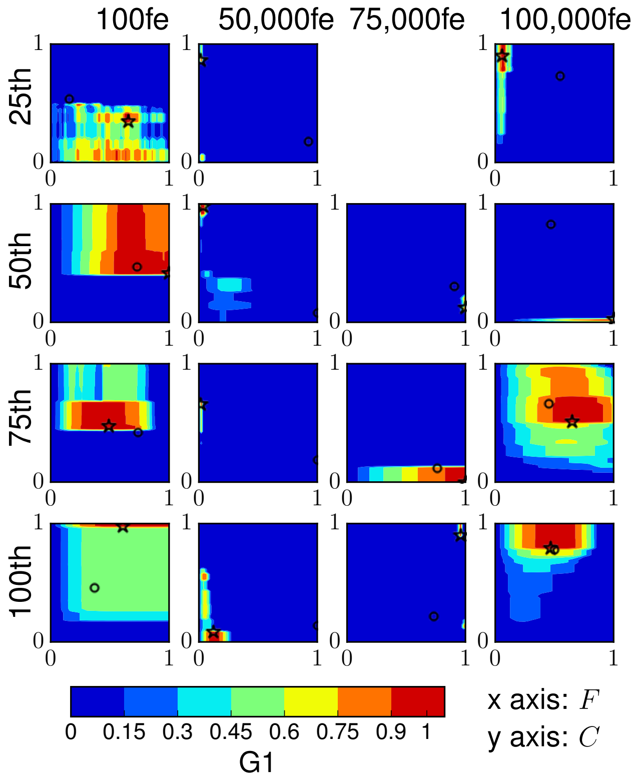


**Figure S.52: Contour maps of adaptive parameter landscapes in P-SHADE on $f_4$ with $d$ = 20.**

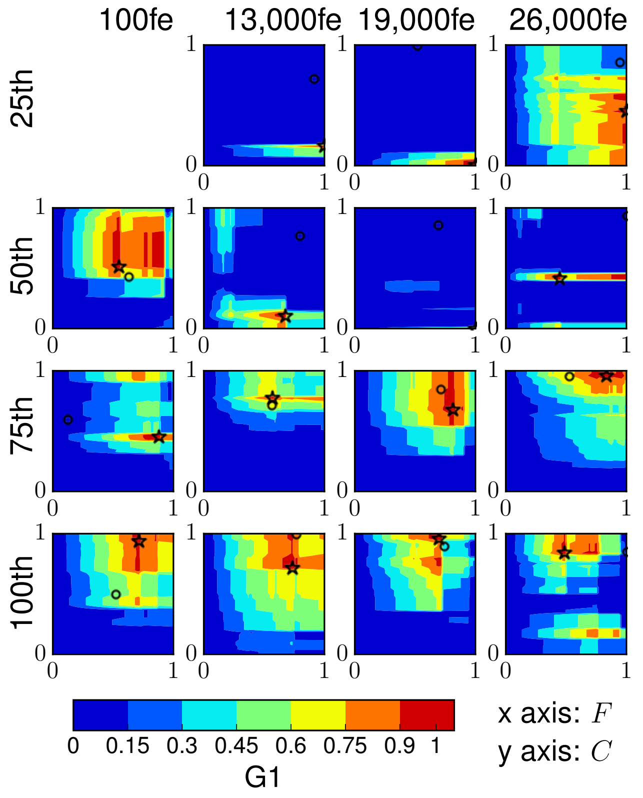


**Figure S.53: Contour maps of adaptive parameter landscapes in P-SHADE on $f_5$ with $d = 20$.**

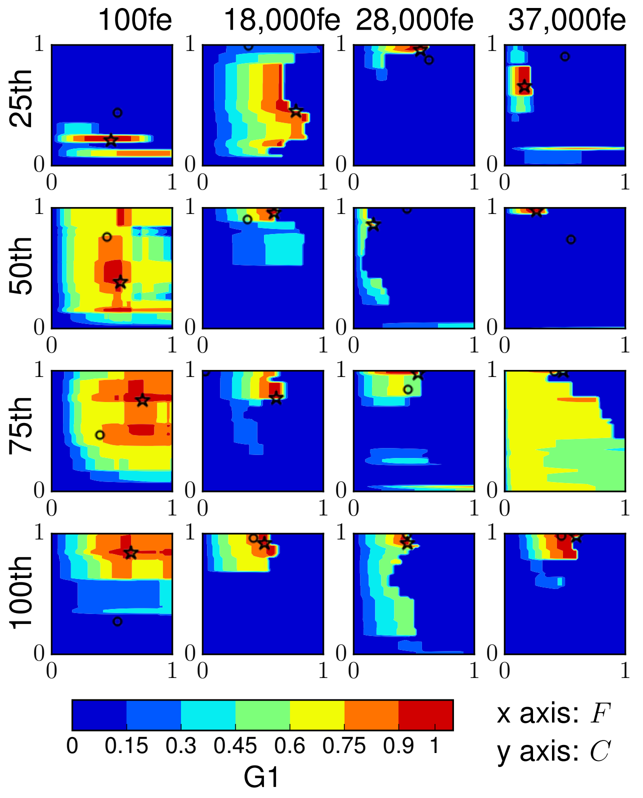


**Figure S.54: Contour maps of adaptive parameter landscapes in P-SHADE on $f_6$ with $d = 20$.**

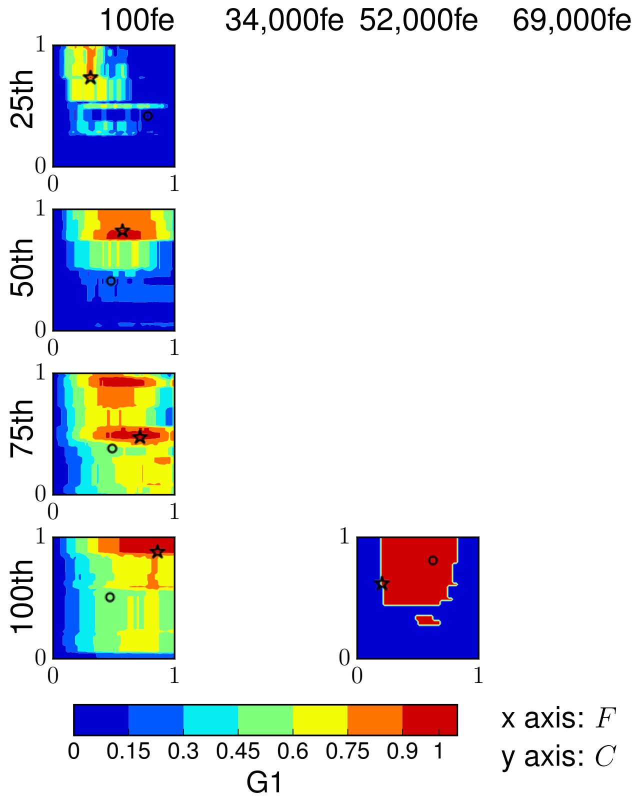


**Figure S.55: Contour maps of adaptive parameter landscapes in P-SHADE on $f_7$ with $d = 20$.**

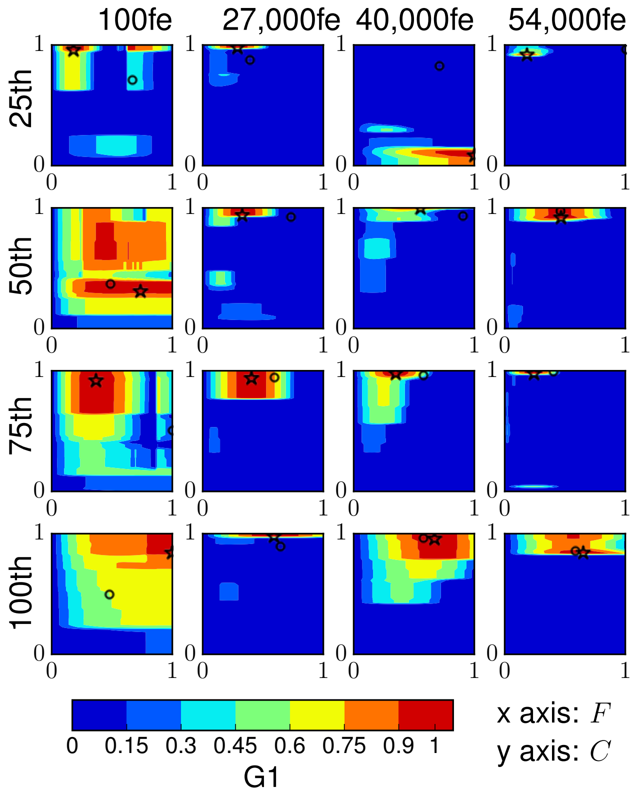


**Figure S.56: Contour maps of adaptive parameter landscapes in P-SHADE on $f_8$ with $d = 20$.**

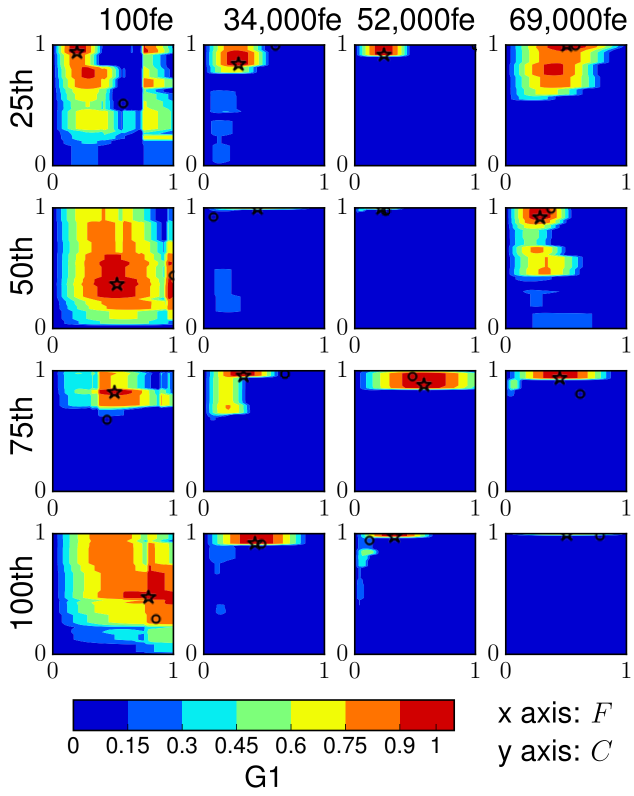


**Figure S.57: Contour maps of adaptive parameter landscapes in P-SHADE on $f_9$ with $d = 20$.**

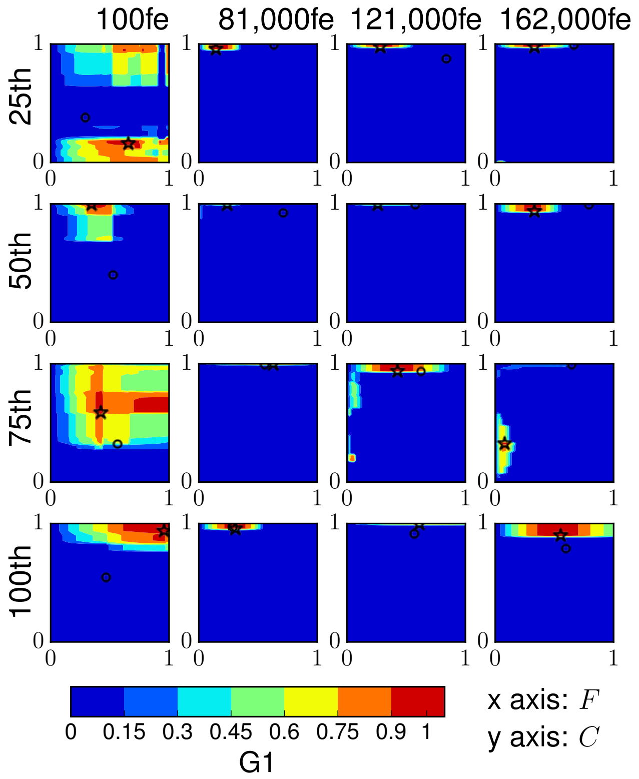


**Figure S.58: Contour maps of adaptive parameter landscapes in P-SHADE on $f_{10}$ with $d = 20$.**

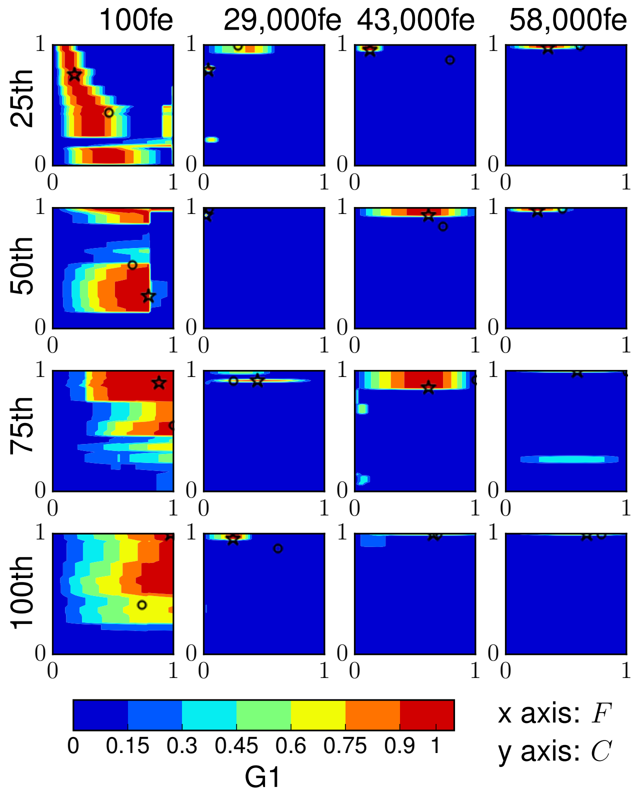


**Figure S.59: Contour maps of adaptive parameter landscapes in P-SHADE on $f_{11}$ with $d = 20$.**

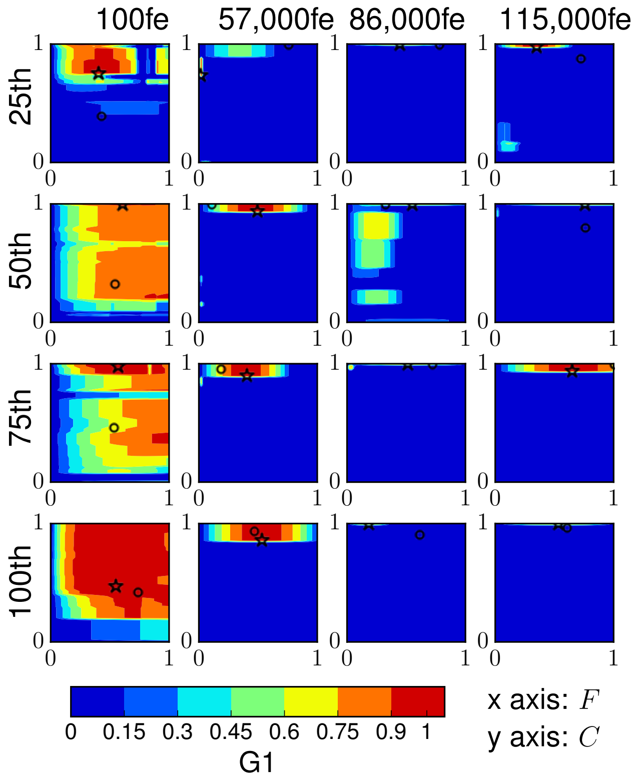


**Figure S.60: Contour maps of adaptive parameter landscapes in P-SHADE on $f_{12}$ with $d = 20$.**

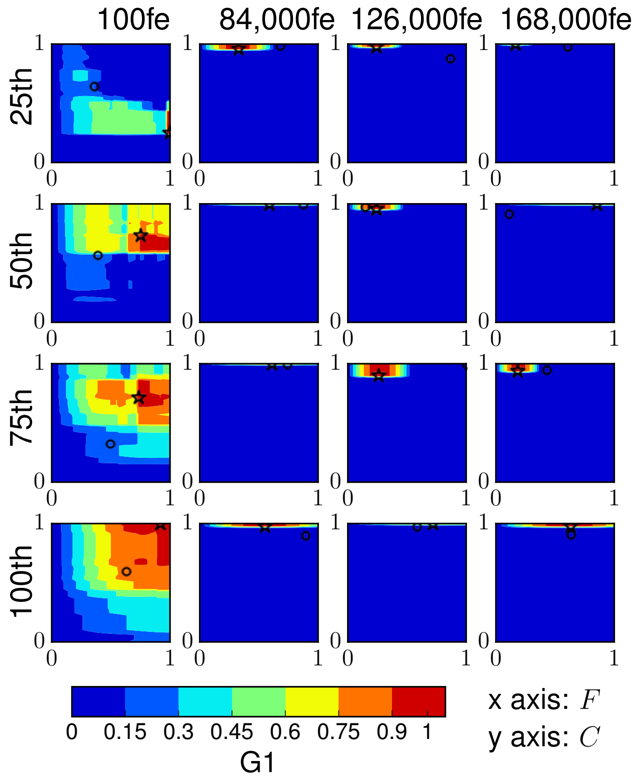


**Figure S.61: Contour maps of adaptive parameter landscapes in P-SHADE on $f_{13}$ with $d = 20$.**

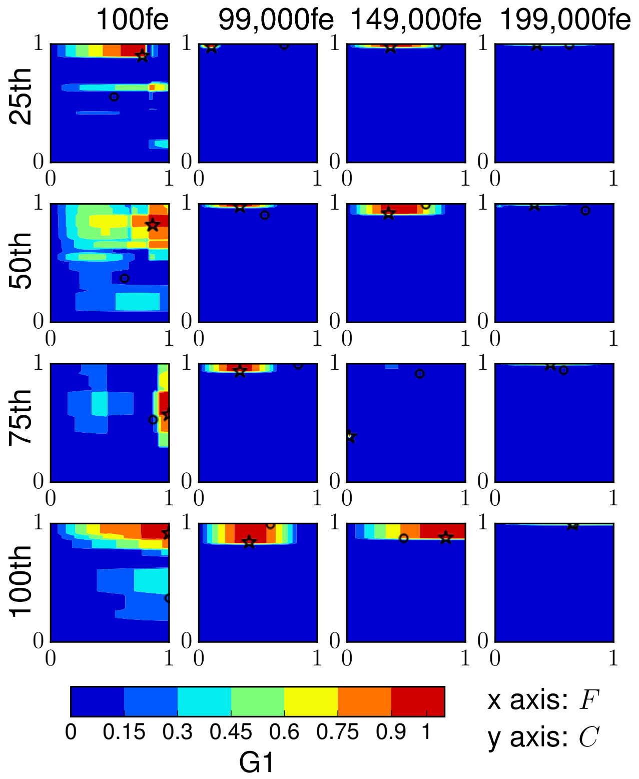


**Figure S.62: Contour maps of adaptive parameter landscapes in P-SHADE on $f_{14}$ with $d = 20$.**

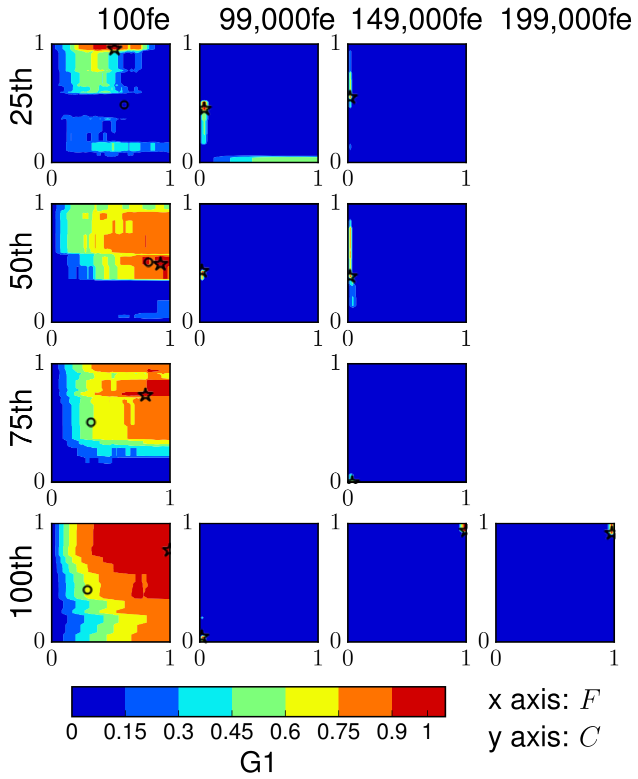


**Figure S.63: Contour maps of adaptive parameter landscapes in P-SHADE on $f_{15}$ with $d = 20$.**

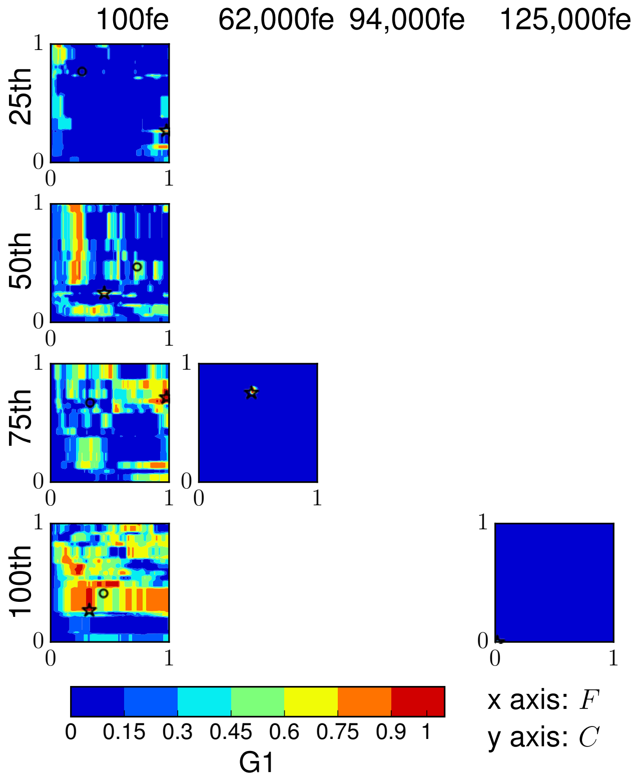


**Figure S.64: Contour maps of adaptive parameter landscapes in P-SHADE on $f_{16}$ with $d = 20$.**

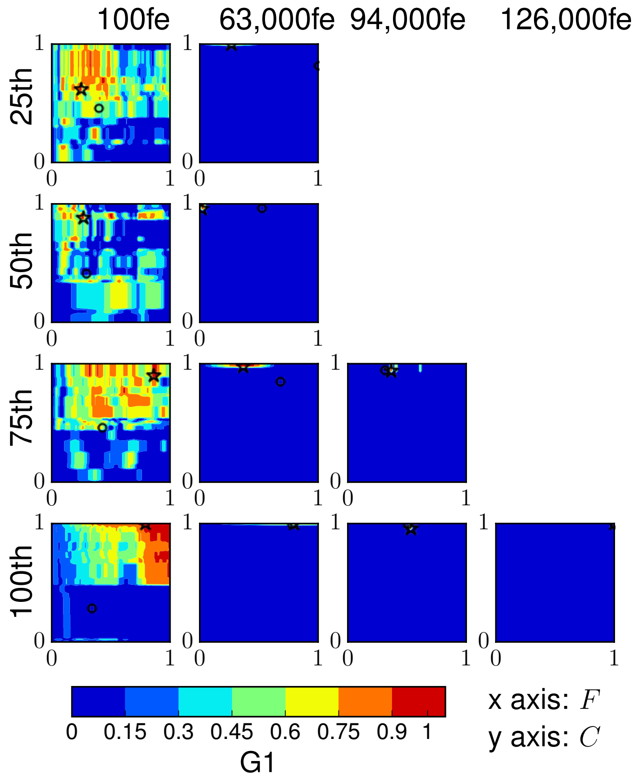


**Figure S.65: Contour maps of adaptive parameter landscapes in P-SHADE on $f_{17}$ with $d = 20$.**

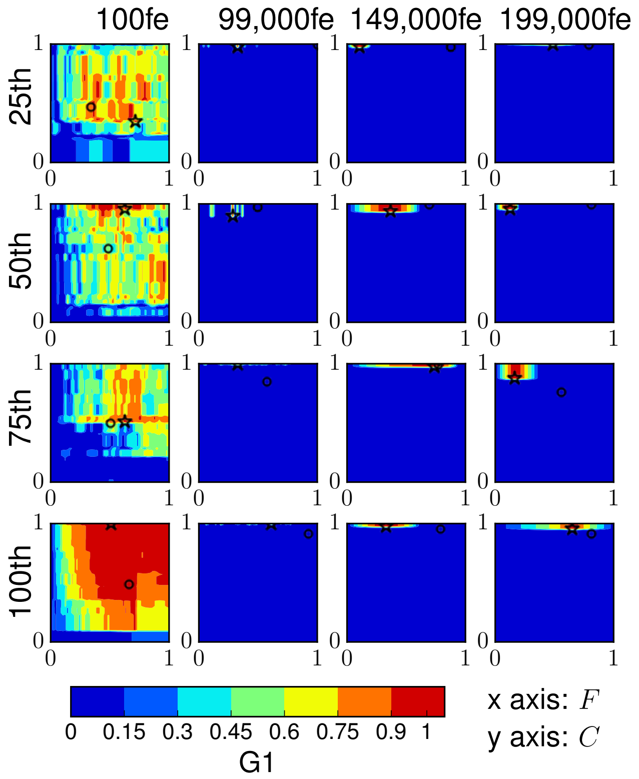


**Figure S.66: Contour maps of adaptive parameter landscapes in P-SHADE on $f_{18}$ with $d = 20$.**

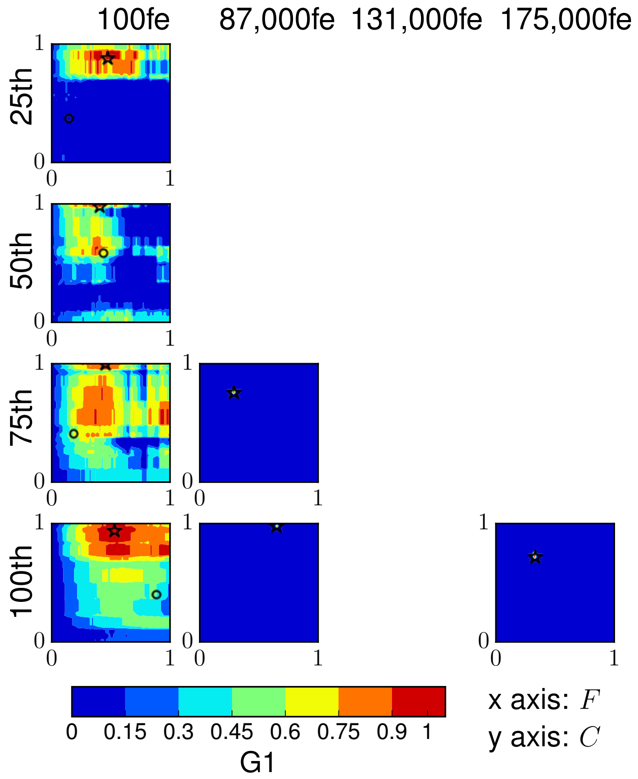


**Figure S.67: Contour maps of adaptive parameter landscapes in P-SHADE on $f_{19}$ with $d = 20$.**

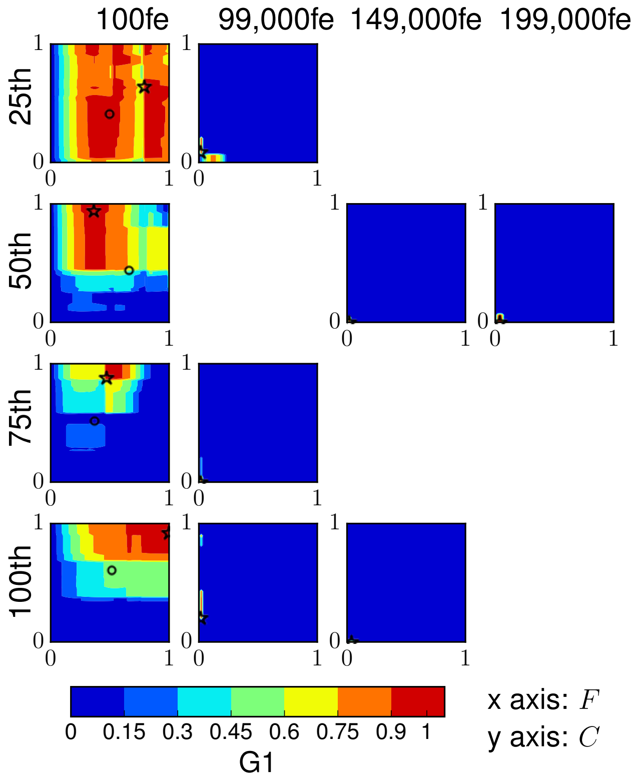


**Figure S.68: Contour maps of adaptive parameter landscapes in P-SHADE on $f_{20}$ with $d = 20$.**

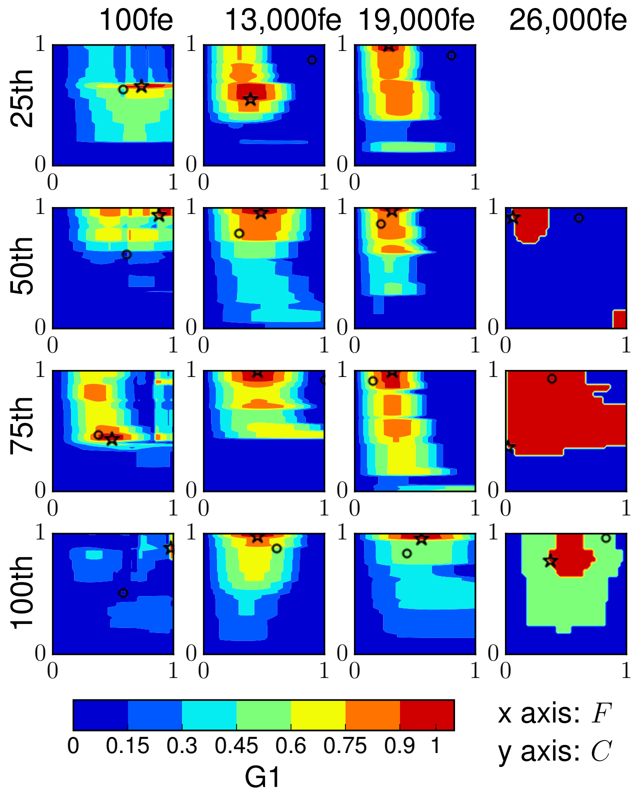


**Figure S.69: Contour maps of adaptive parameter landscapes in P-SHADE on $f_{21}$ with $d = 20$.**

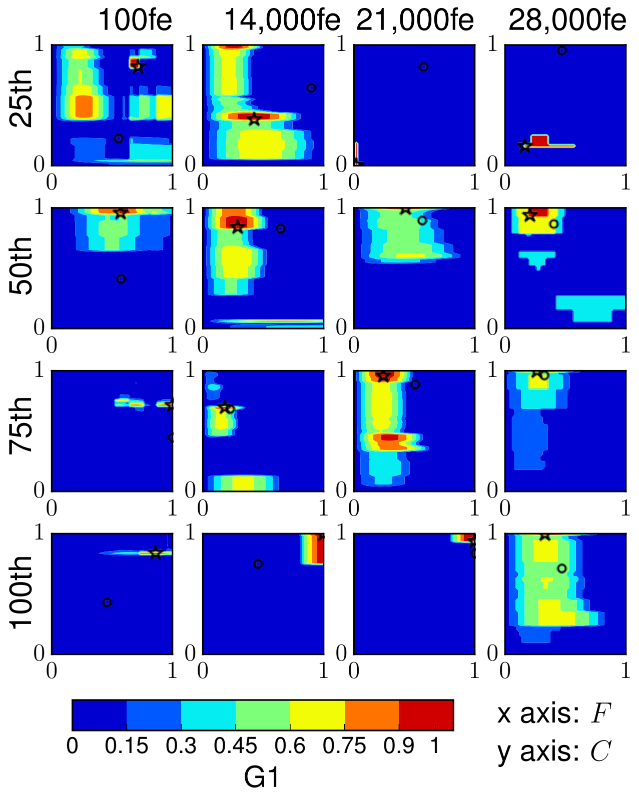


**Figure S.70: Contour maps of adaptive parameter landscapes in P-SHADE on $f_{22}$ with $d = 20$.**

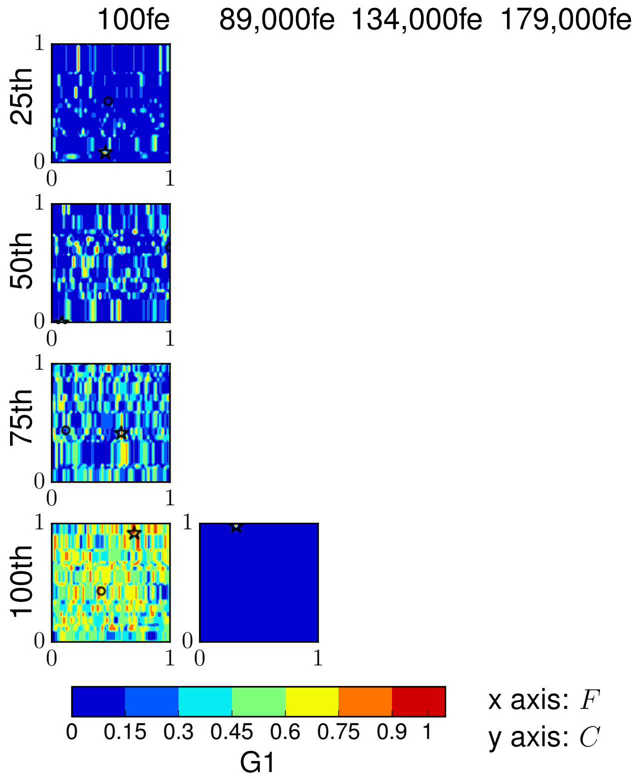


**Figure S.71: Contour maps of adaptive parameter landscapes in P-SHADE on $f_{23}$ with $d = 20$.**

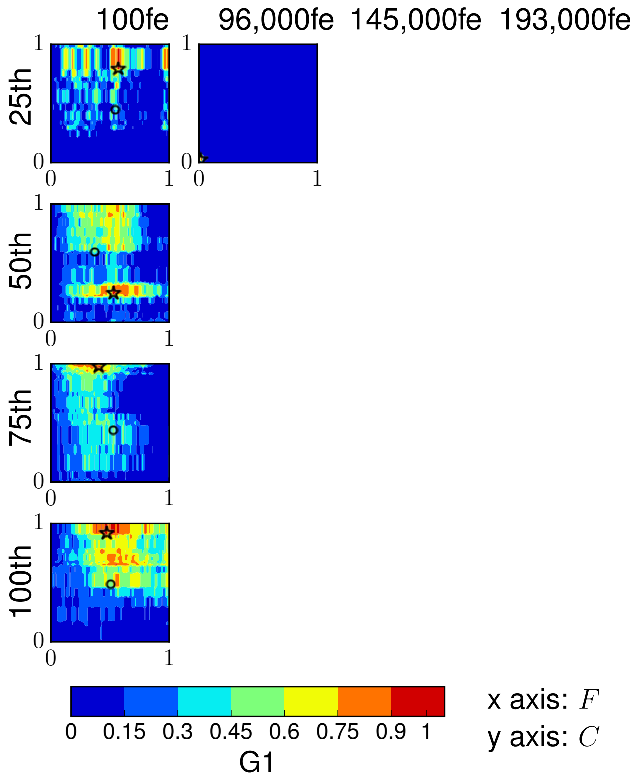


**Figure S.72: Contour maps of adaptive parameter landscapes in P-SHADE on $f_{24}$ with $d = 20$.**

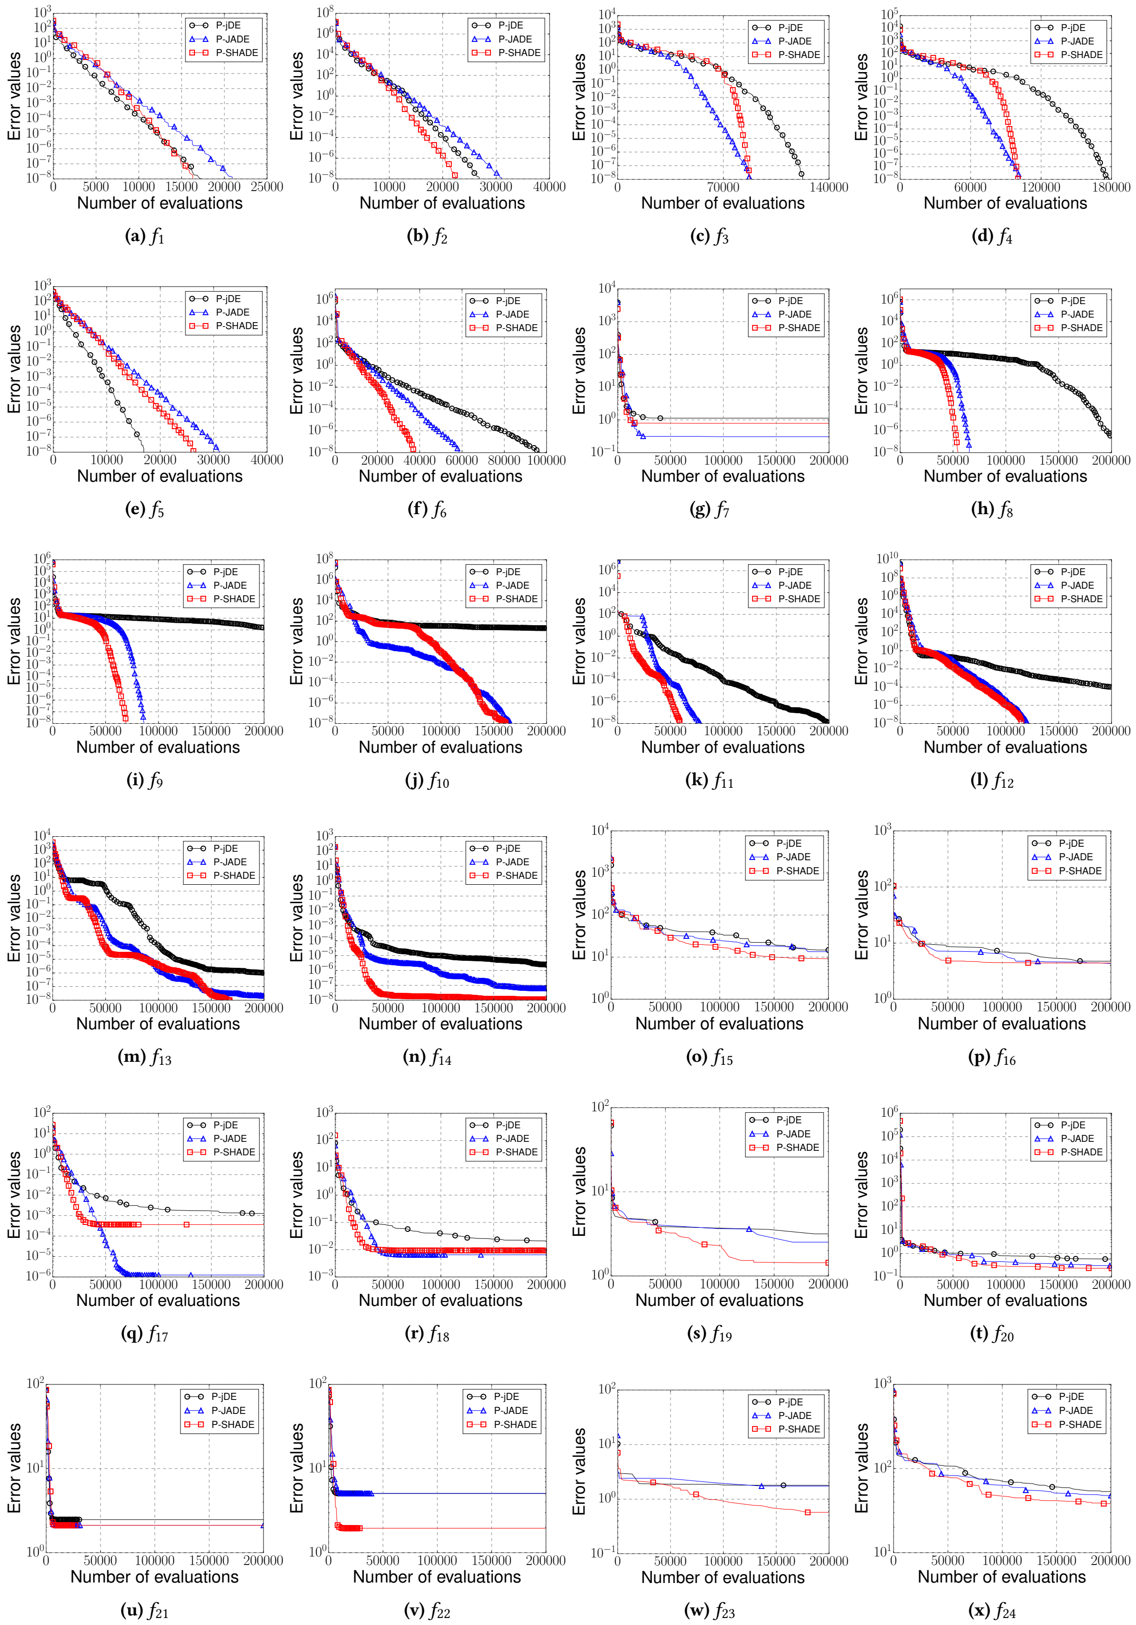


**(a)** $f_1$ **(b)** $f_2$ **(c)** $f_3$ **(d)** $f_4$

**(e)** $f_5$ **(f)** $f_6$ **(g)** $f_7$ **(h)** $f_8$

**(i)** $f_9$ **(j)** $f_{10}$ **(k)** $f_{11}$ **(l)** $f_{12}$

**(m)** $f_{13}$ **(n)** $f_{14}$ **(o)** $f_{15}$ **(p)** $f_{16}$

**(q)** $f_{17}$ **(r)** $f_{18}$ **(s)** $f_{19}$ **(t)** $f_{20}$

**(u)** $f_{21}$ **(v)** $f_{22}$ **(w)** $f_{23}$ **(x)** $f_{24}$

**Figure S.73: Error values of DE with P-jDE, P-JADE, and P-SHADE on the 24 BBOB functions with $d = 20$.**

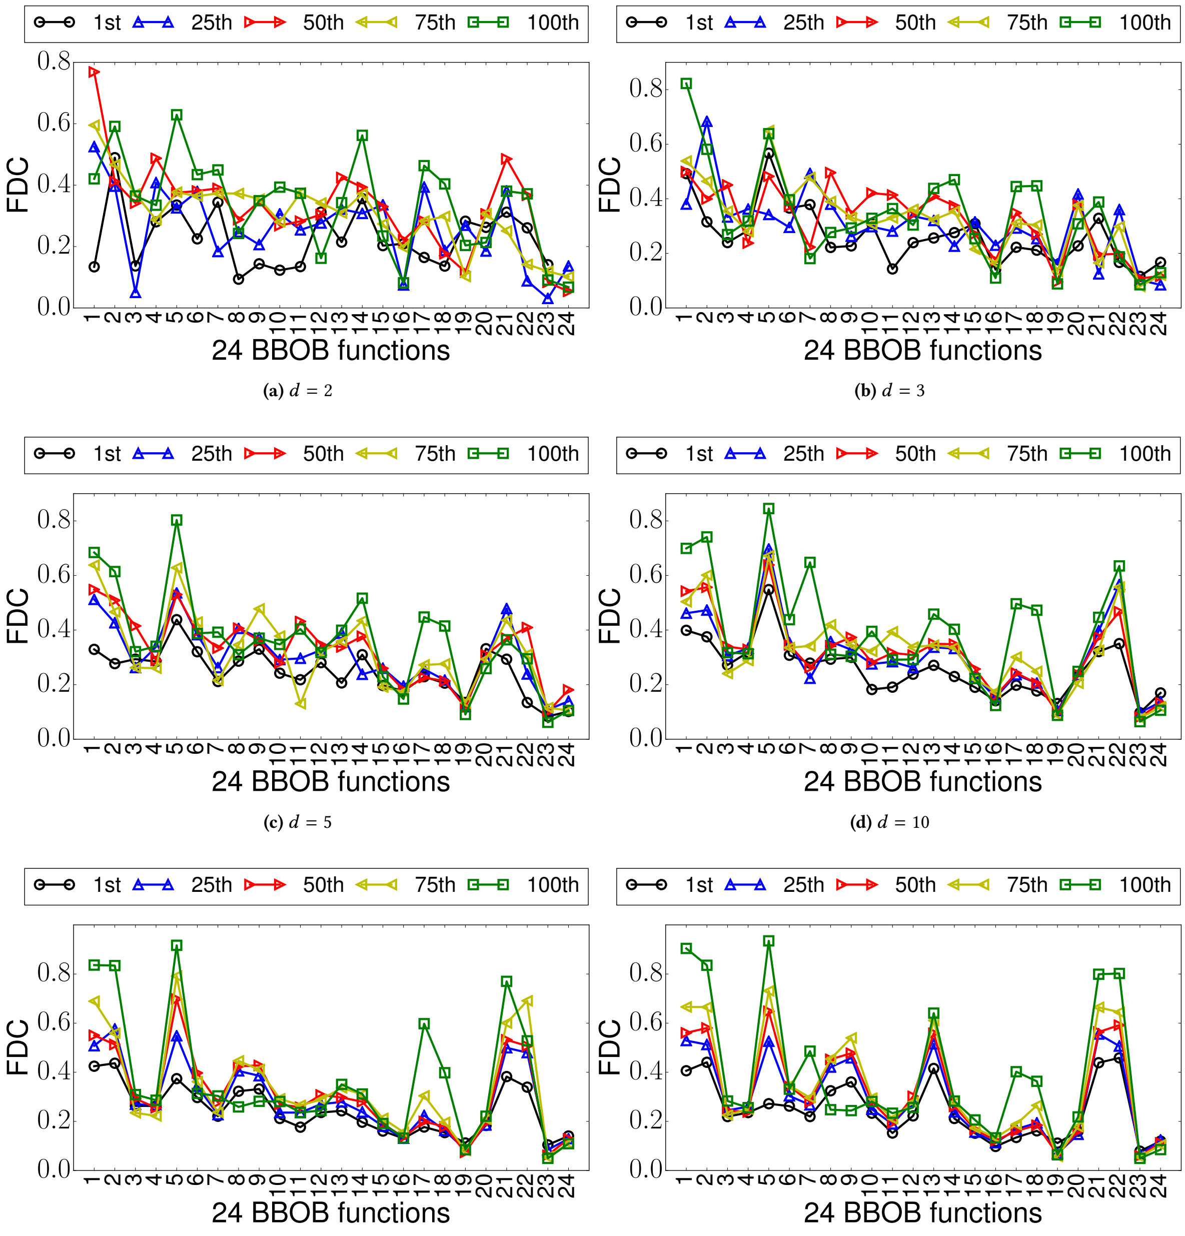


(a) $d = 2$

(b) $d = 3$

(c) $d = 5$

(d) $d = 10$

(e) $d = 20$

(f) $d = 40$

**Figure S.74: Average FDC values of P-jDE on the 24 BBOB functions with $d \in \{2, 3, 5, 10, 20, 40\}$.**

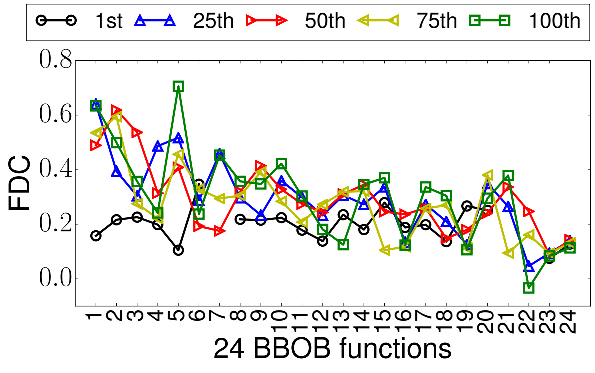


(a) $d = 2$

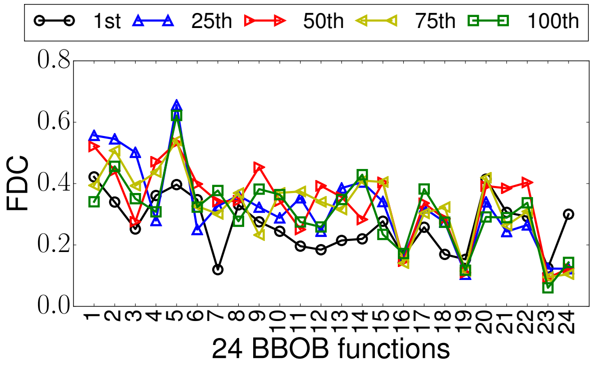


(b) $d = 3$

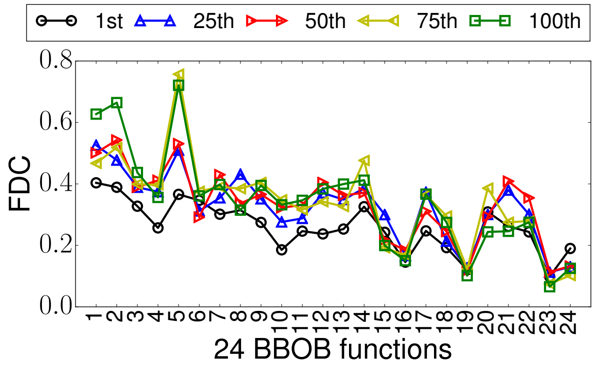


(c) $d = 5$

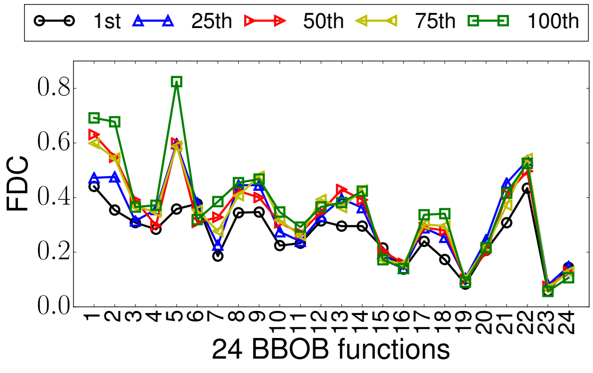


(d) $d = 10$

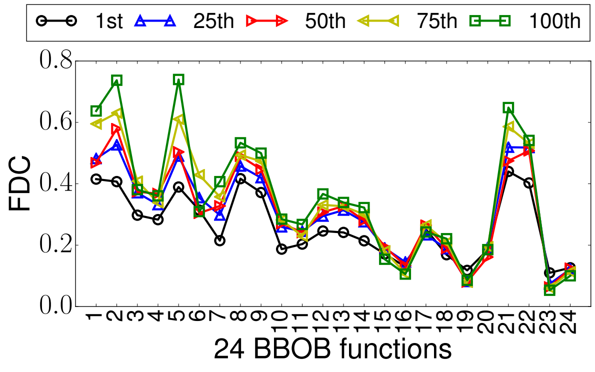


(e) $d = 20$

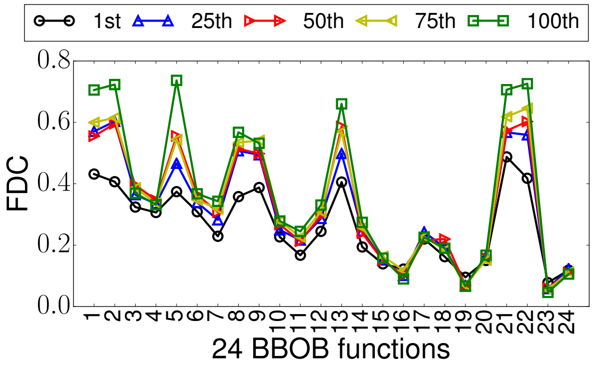


(f) $d = 40$

**Figure S.75: Average FDC values of P-JADE on the 24 BBOB functions with $d \in \{2, 3, 5, 10, 20, 40\}$.**

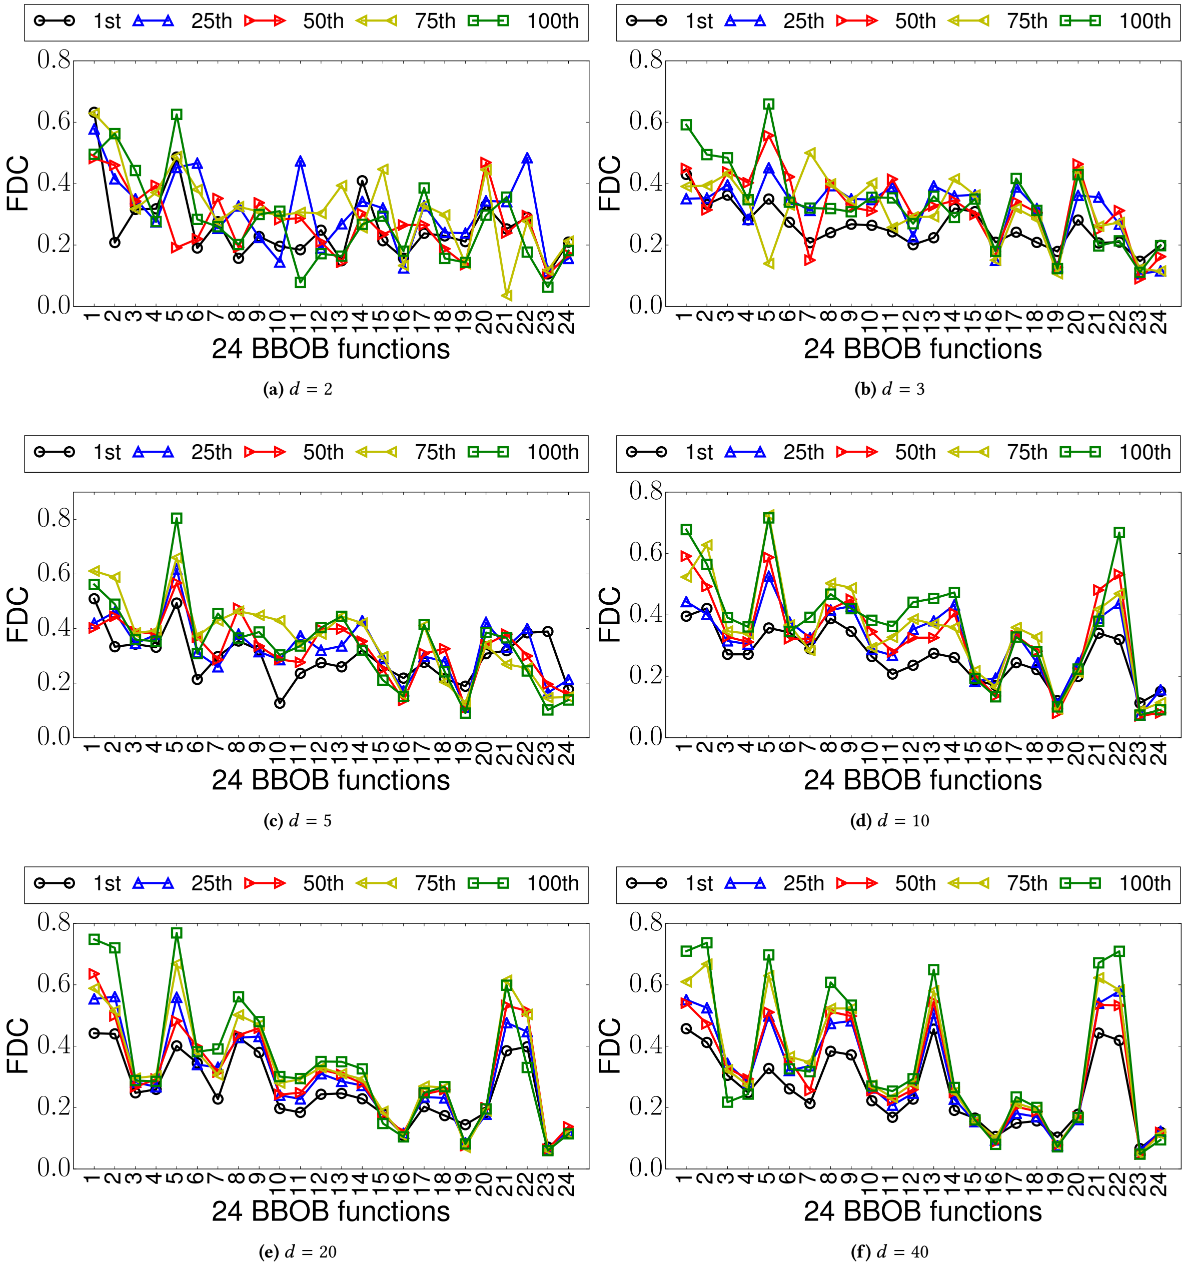


(a) $d = 2$ (b) $d = 3$ (c) $d = 5$ (d) $d = 10$ (e) $d = 20$ (f) $d = 40$

**Figure S.76: Average FDC values of P-SHADE on the 24 BBOB functions with $d \in \{2, 3, 5, 10, 20, 40\}$.**

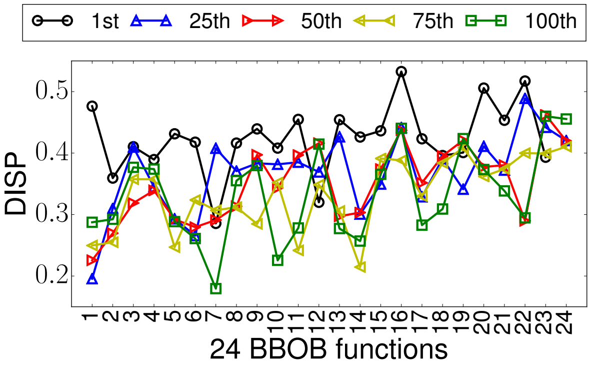


**(a)** $d = 2$

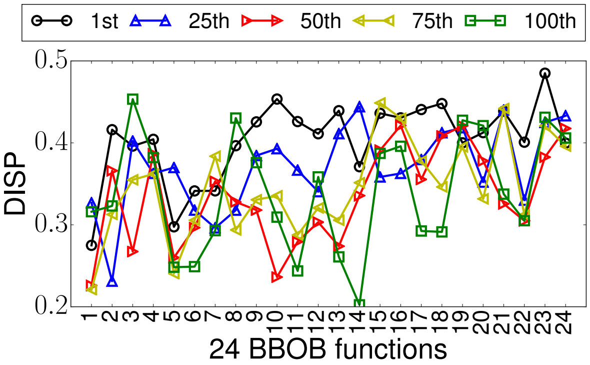


**(b)** $d = 3$

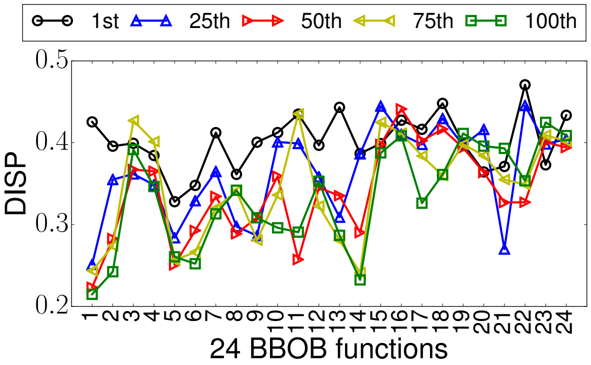


**(c)** $d = 5$

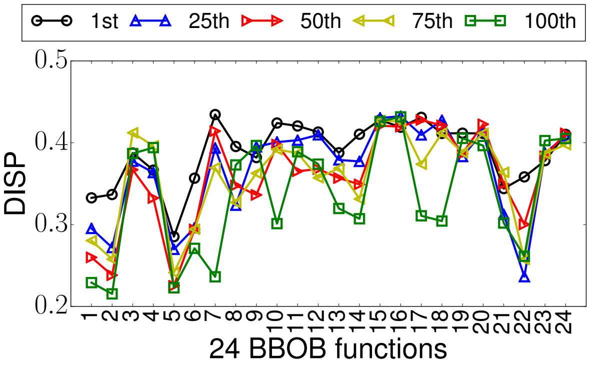


**(d)** $d = 10$

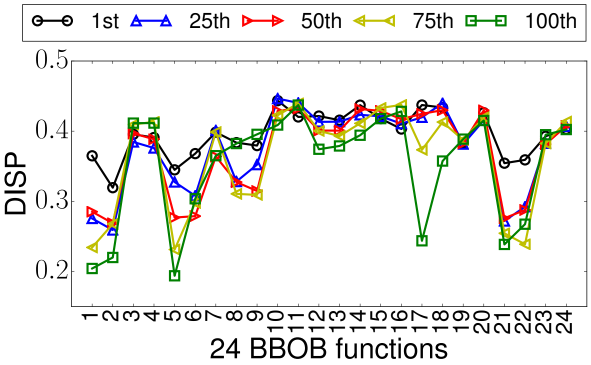


**(e)** $d = 20$

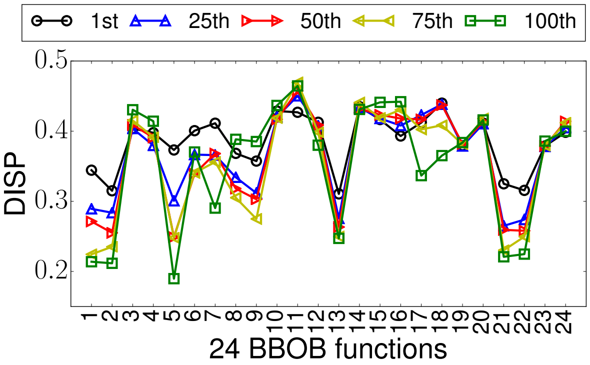


**(f)** $d = 40$

**Figure S.77: Average DISP values of P-jDE on the 24 BBOB functions with $d \in \{2, 3, 5, 10, 20, 40\}$.**

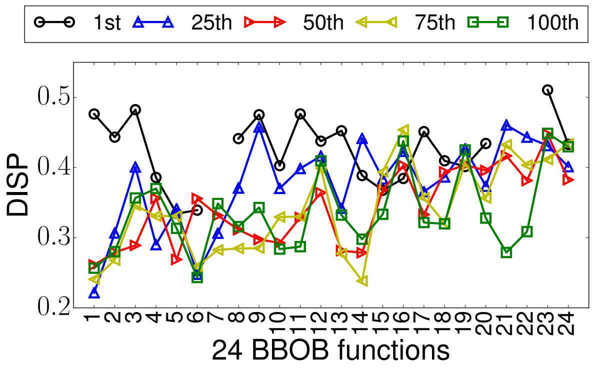


(a) $d = 2$

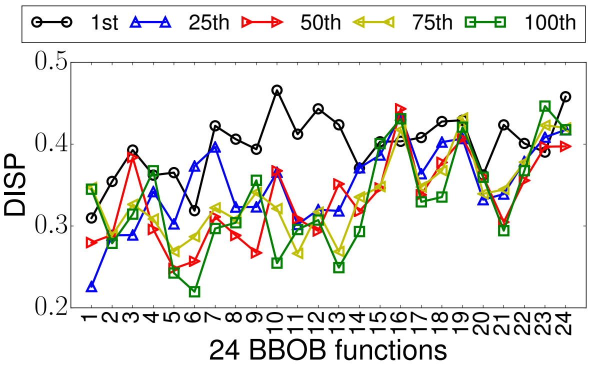


(b) $d = 3$

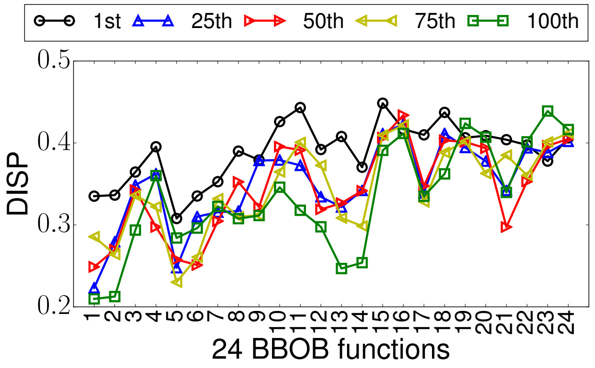


(c) $d = 5$

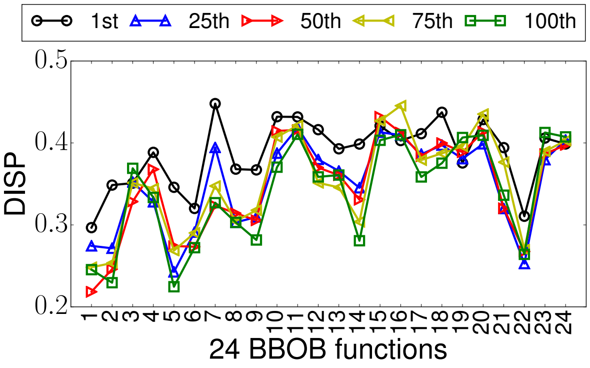


(d) $d = 10$

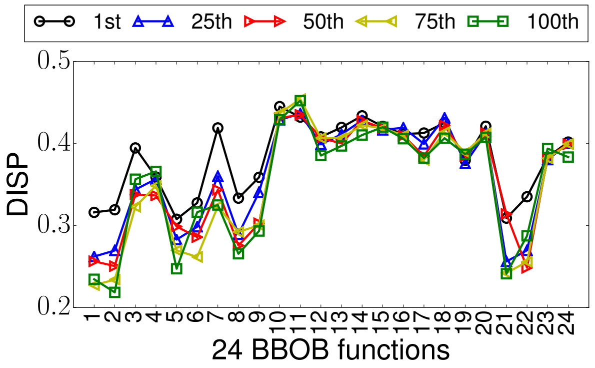


(e) $d = 20$

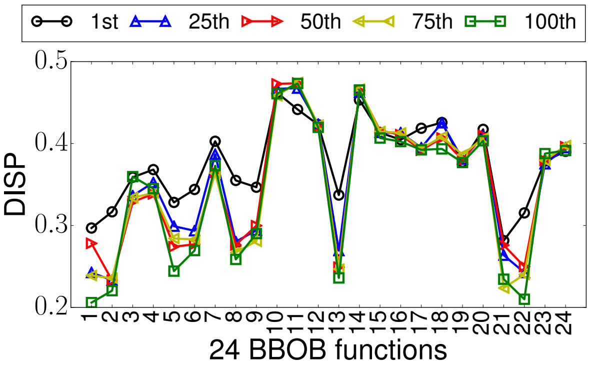


(f) $d = 40$

**Figure S.78: Average DISP values of P-JADE on the 24 BBOB functions with $d \in \{2, 3, 5, 10, 20, 40\}$.**

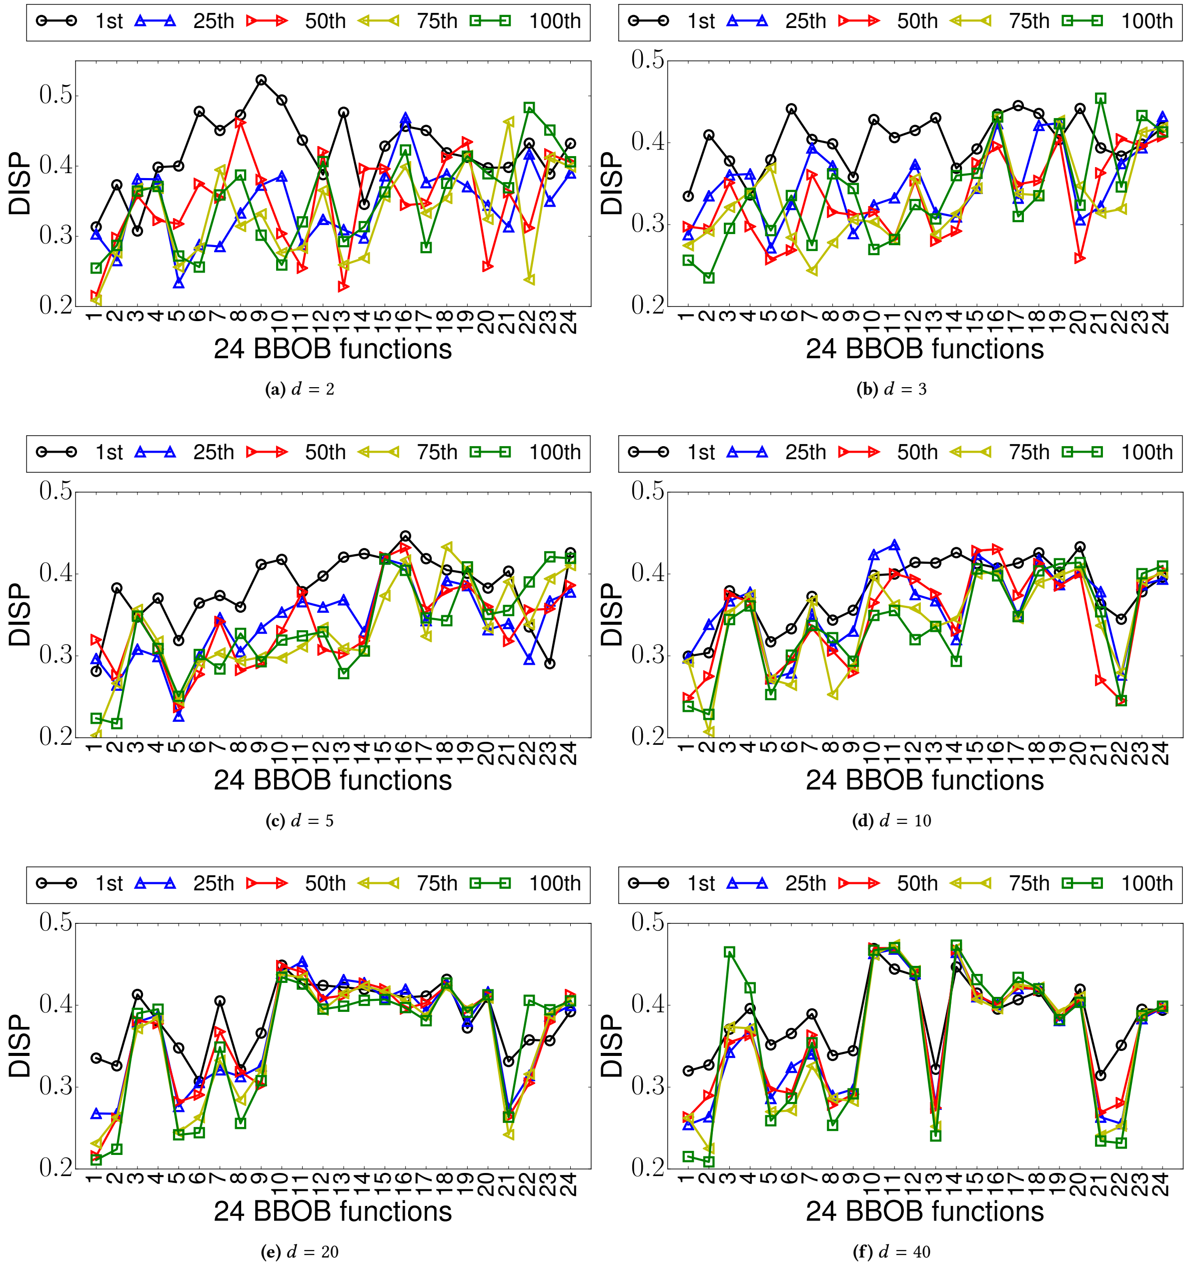


**Figure S.79: Average DISP values of P-SHADE on the 24 BBOB functions with $d \in \{2, 3, 5, 10, 20, 40\}$.**

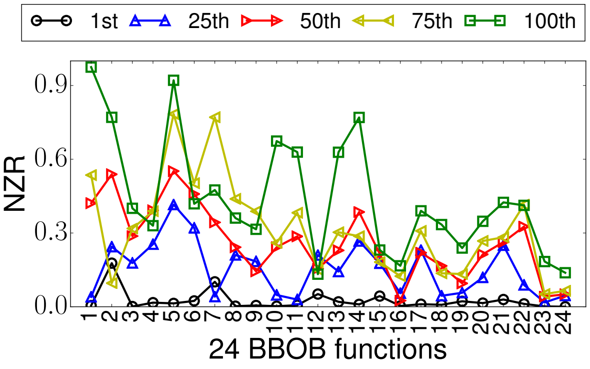


(a) $d = 2$

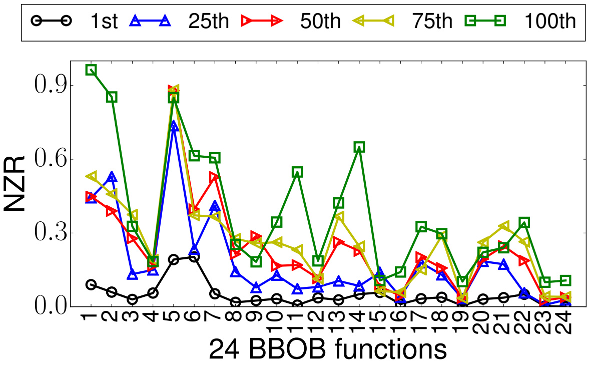


(b) $d = 3$

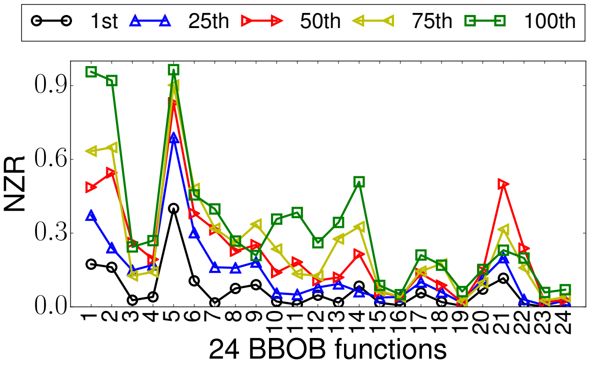


(c) $d = 5$

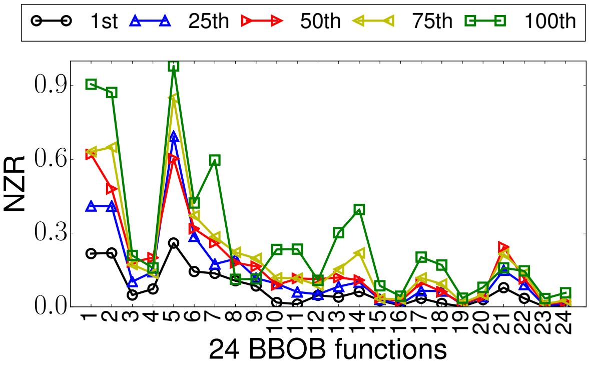


(d) $d = 10$

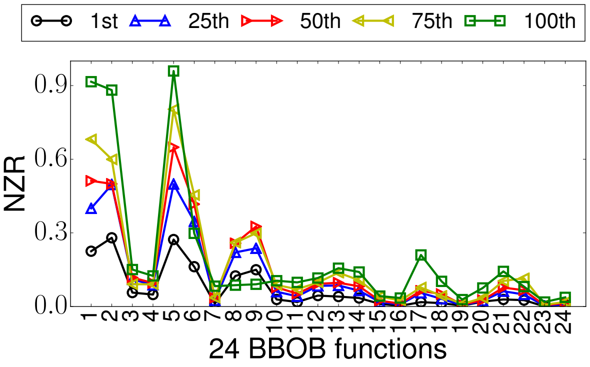


(e) $d = 20$

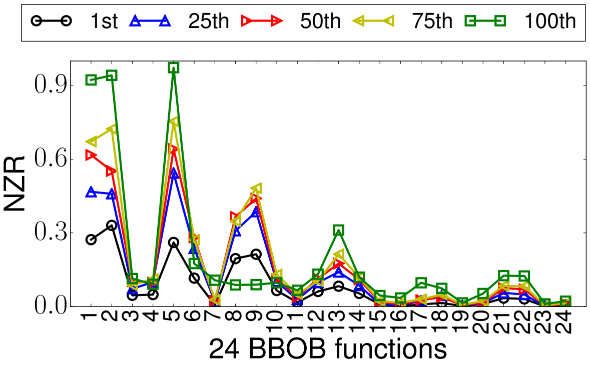


(f) $d = 40$

**Figure S.80: Average NZR values of P-jDE on the 24 BBOB functions with $d \in \{2, 3, 5, 10, 20, 40\}$.**

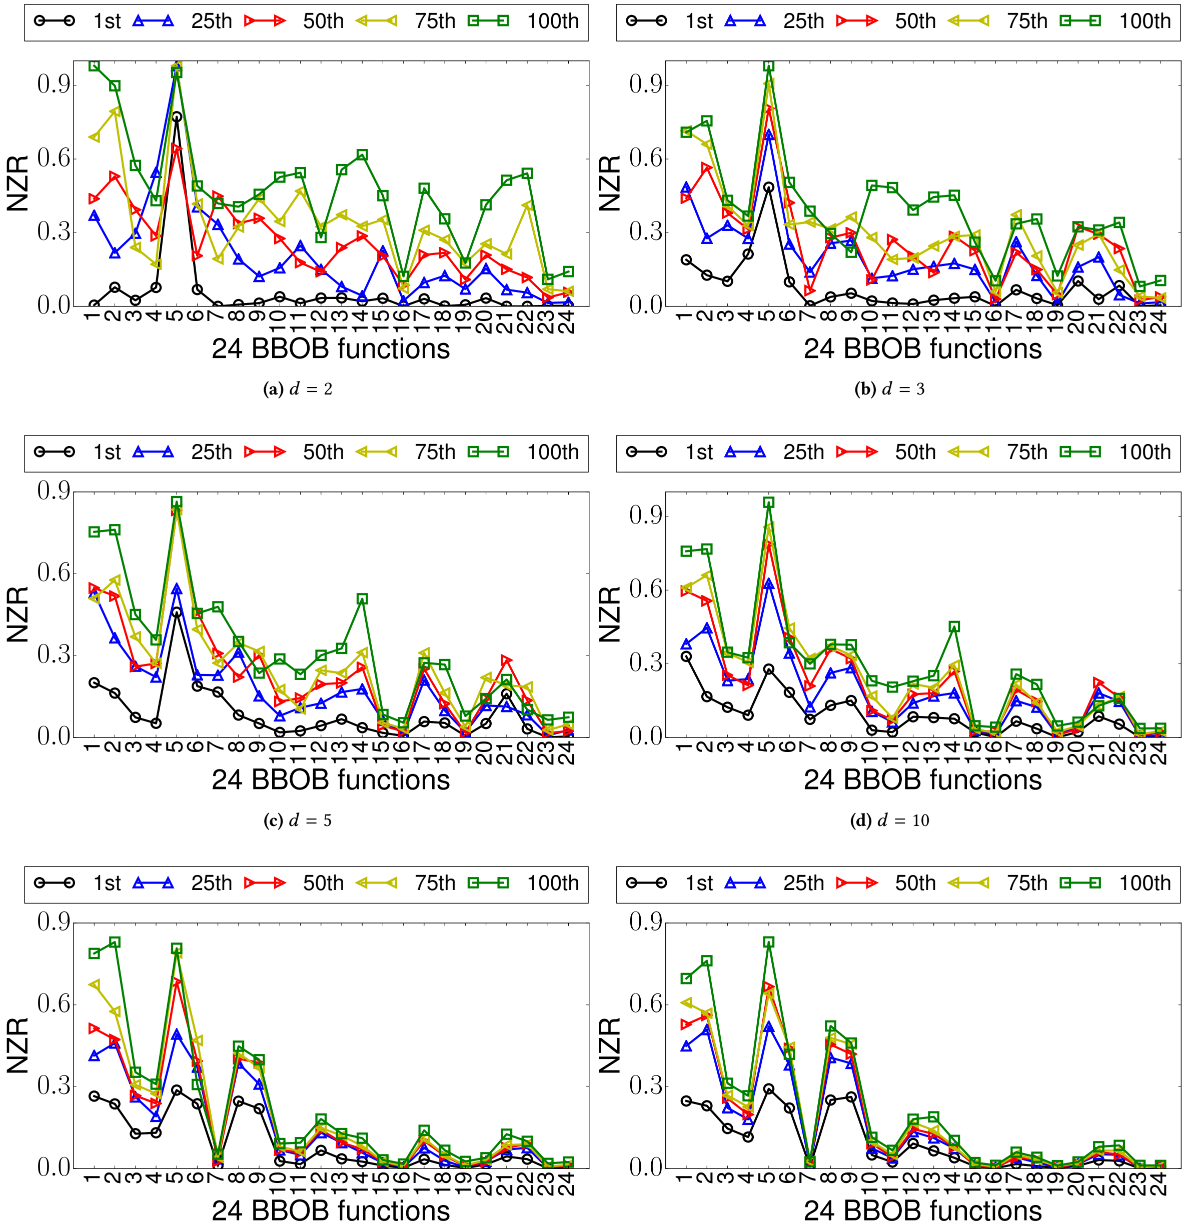


(a) $d = 2$ (b) $d = 3$

(c) $d = 5$ (d) $d = 10$

(e) $d = 20$ (f) $d = 40$

**Figure S.81: Average NZR values of P-JADE on the 24 BBOB functions with $d \in \{2, 3, 5, 10, 20, 40\}$.**

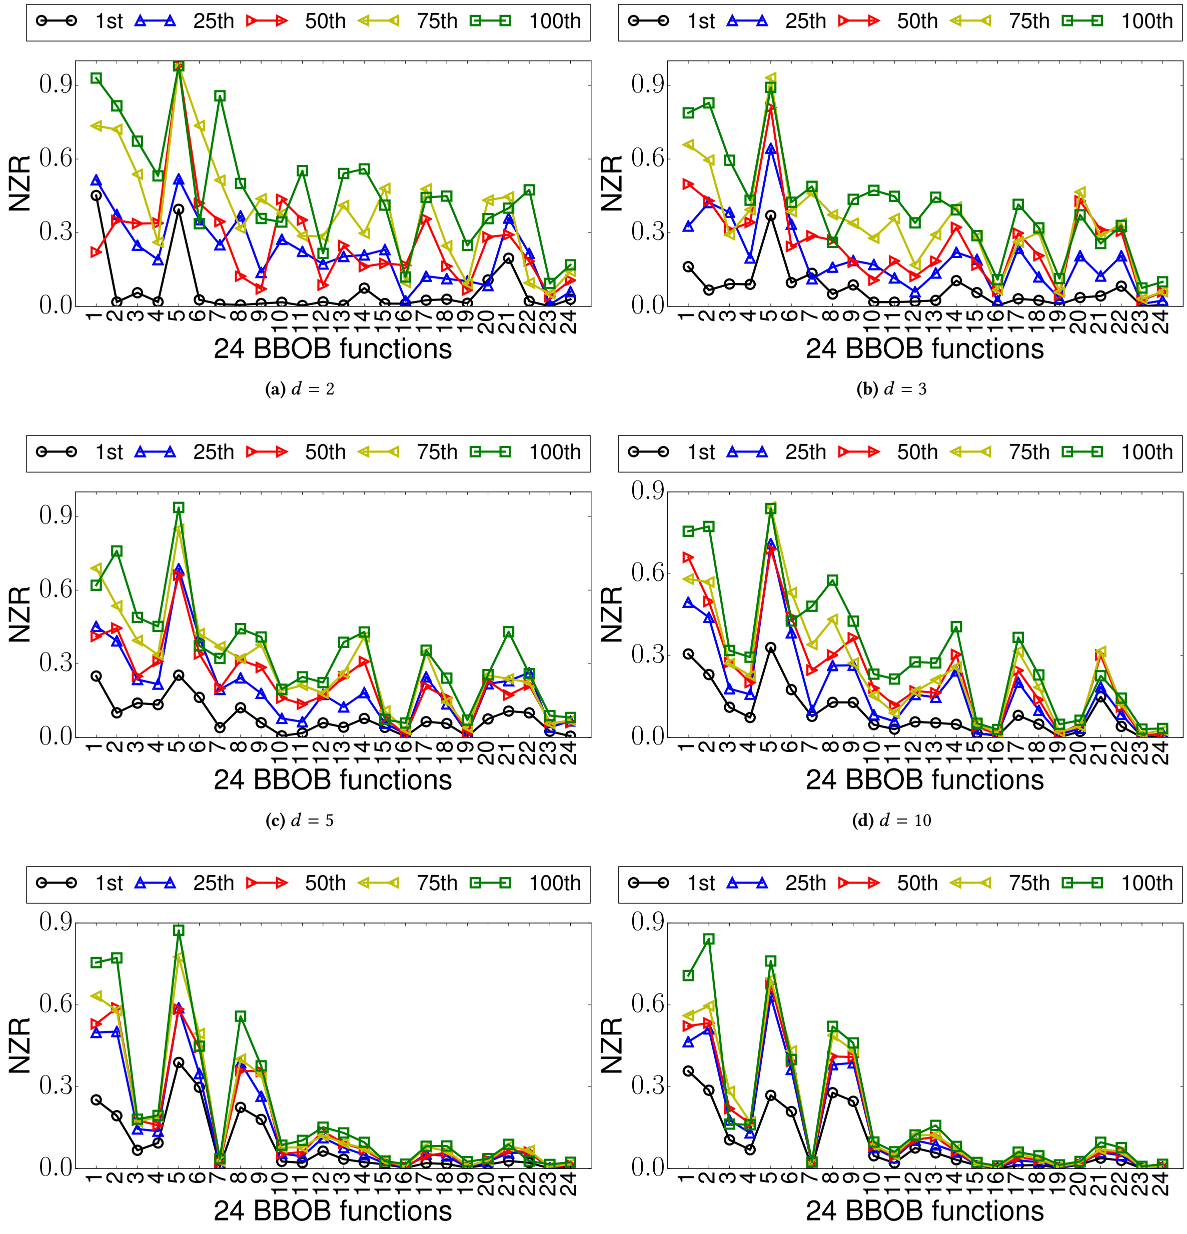


(a) $d = 2$

(b) $d = 3$

(c) $d = 5$

(d) $d = 10$

(e) $d = 20$

(f) $d = 40$

**Figure S.82: Average NZR values of P-SHADE on the 24 BBOB functions with $d \in \{2, 3, 5, 10, 20, 40\}$.**
